# Supplementary material for: Decoupling of Spin Decoherence Paths near Zero Magnetic Field
Source: arXiv:2112.08536 source file (2021-12-16)
Supplement: Supplementary file 1 [file SupportingInformation.pdf]

# Decoupling of Spin Decoherence Paths Near Zero Magnetic Field

### Supporting Information

**Sven Bodenstedt[a], Denis Moll[b,c], Stefan Glöggler[b,c], Morgan W. Mitchell[a,d], Michael C. D. Tayler[a,*]**

[a] *ICFO-Institut de Ciències Fotòniques, The Barcelona Institute of Science and Technology, 08860 Castelldefels (Barcelona), Spain.*

[b] *NMR Signal Enhancement Group, Max Planck Institute for Biophysical Chemistry, 37077 Göttingen, Germany.*

[c] *Center for Biostructural Imaging of Neurodegeneration, UMG, 37075 Göttingen, Germany.*

[d] *ICREA – Institució Catalana de Recerca i Estudis Avançats, 08010 Barcelona, Spain.*

[*] *Corresponding author. Email: michael dot tayler at icfo dot eu*

## Contents

S.1 Sample Preparation .......... 2
S.2 DC Pulse Length Calibration .......... 3
S.3 Experimental Benchmarking of Composite $\pi$-Pulse .......... 4
S.4 Experimental Benchmarking of XY4 Phase Cycling .......... 6
S.5 Shimming Procedure .......... 7
S.6 Spin Dynamics Simulations .......... 8

## S.1 Sample Preparation

### Water

High-purity (milli-Q) water was used without further treatment.

### [2,2,2-d$_3$]-Ethanol ($CD_3CH_2OH$)

The compound was obtained commercially as a liquid (99 % isotopic purity, Sigma-Aldrich product 329347, CAS 1759-87-1) and degassed by bubbling argon for 2 to 3 minutes. The degassing procedure was used to displace dissolved paramagnetic $O_2$, which can otherwise act as a source of relaxation.

### Pyrazine ($C_4H_4N_2$)

The compound was obtained commercially (Sigma Aldrich product P56003, CAS 290-37-9) as a crystalline solid. The solid was dissolved in deuterated water ($D_2O$) to a concentration of 2 mol/dm$^3$ then degassed by argon bubbling.

### Tetraalkylammonium Bromide Salts

$NMe_4Br$ (Sigma-Aldrich product 195758, CAS 64-20-0) and $NEt_4Br$ (Sigma-Aldrich product 140023, CAS 71-91-0) were obtained commercially. The solids were dissolved in deuterated water ($D_2O$) to concentrations of 3.2 mol/dm$^3$ and 2.5 mol/dm$^3$ respectively.

$NEtMe_3Br$ was synthesized chemically via the following protocol

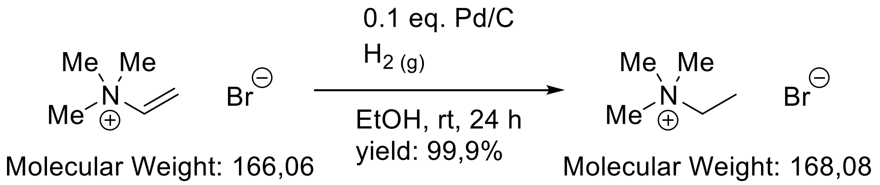


*Synthesis*: Trimethylvinylammonium bromide 1 g, 6.0 mmol, 1 eq.) was dissolved in EtOH (50 mL) in a flask. Pd/C (0.064 g, 0.6 mmol, 0.1 eq.) was then added under inert conditions and the pressure reduced before bubbling $H_2$ through the solution by using a balloon attached to a syringe. The balloon was re-filled a total of three times and the reaction mixture was then stirred at room temperature for 24 h. A crude solid product was filtered through a Celite pad and concentrated under reduced pressure giving pure trimethylethylammonium bromide salt in 99.9 % yield (1 g).

Purity was confirmed via $^1$H NMR (see Figure 1) at 300 MHz ($CDCl_3$): $\delta = 3.75$ ppm (q, $^3J_{\mathrm{HH}} = 7.29$ Hz, 2 H), $\delta = 3.45$ ppm (s, 9 H), $\delta = 1.44$ ppm (tt, $^3J_{\mathrm{HH}} = 7.29$ Hz, $^2J_{\mathrm{NH}} = 1.9$ Hz, 3 H).

Solid $NEtMe_3Br$ was then dissolved to a concentration of 3.0 mol/dm$^3$ in $D_2O$.

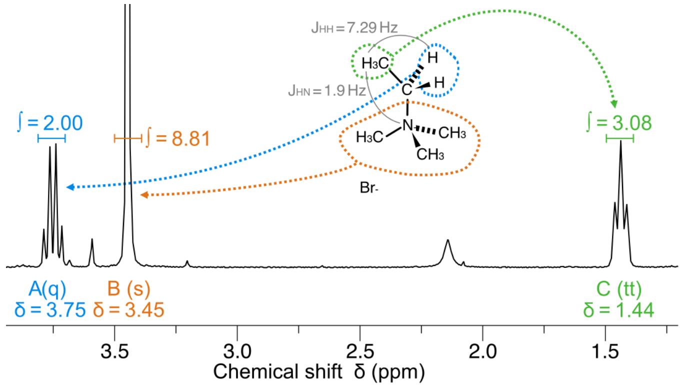


Figure 1: $^1$H NMR spectrum of $^{14}$NEtMe$_3$Br at 7.0 T, with horizontal axis in units of $^1$H chemical shift (frequency 300 Hz/ppm)

## S.2 DC Pulse Length Calibration

Calibration of the field to-current ratio and homogeneity for each $x$ or $y$ coil was performed using the $H_2O$ sample. After initial prepolarization of the $^1$H spins in a 20 mT field, a rectangular pulse of 1.5 A was applied in one of the coils and after that, the $^1$H free precession signal was recorded. The amplitude of the precession signal was measured for a series of different pulse lengths to obtain a Rabi curve, shown below in Figure 2 for the $x$ coil. One fourth of the Rabi period, or around 46 µs, equals the duration of a $\pi/2$ dc pulse on $^1$H.

The homogeneity of the pulse coils was quantified using the ratio of amplitudes $A$ for the proton precession signal after a $\pi/2$ ($A_{\pi/2}$) and $9 \times \pi/2$ ($A_{9\pi/2}$) pulse; $A_{9\pi/2}/A_{\pi/2}$ was approximately 0.96.

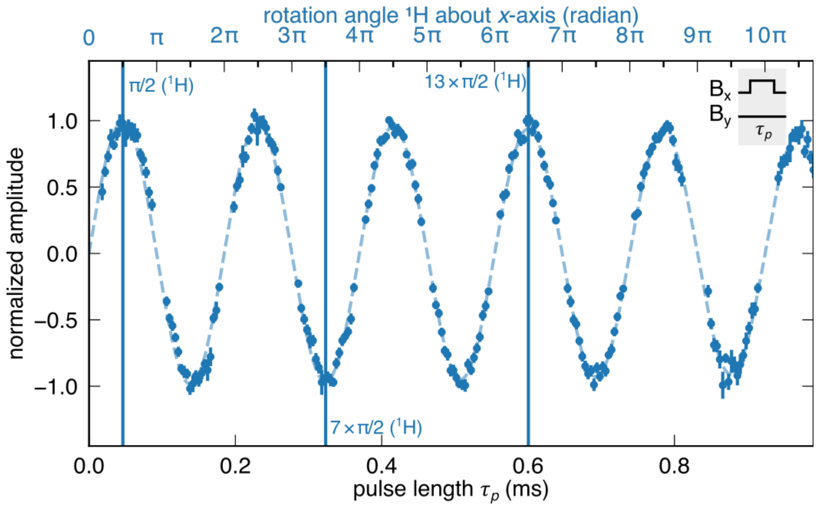


Figure 2: Experimental calibration of dc pulse lengths for the $x$ field coil. Data show relative amplitudes of the proton precession signal after prepolarization followed by a dc magnetic pulse of length $\tau_p$. A sine curve (blue dotted line) fitted to the data gives accurate pulse durations for flip angles of $\pi/2$ (46.48(2) µs), $7 \times \pi/2$ (323.28(2) µs) and $13 \times \pi/2$ (600.38(2) µs) as indicated by the solid vertical lines.

## S.3 Experimental Benchmarking of Composite $\pi$-Pulse

When a dc pulse of flip angle $7\pi$ is applied to $^1$H, the corresponding flip angle on $^2$H is within 7.5 percent of $\pi$, and similarly when the $^1$H flip angle is $13\pi$ the corresponding flip angle on $^{14}$N is within 6.1 percent of $\pi$. To improve the accuracy of $\pi$ rotations needed for XY4(I) and XY4(I+S) sequences, we substitute single rectangular pulses with $(\pi/2)_x - (\pi)_y - (\pi/2)_x$ composite pulses.

Fidelity of composite pulses near to zero field was determined experimentally by field cycling. After initial prepolarization at 20 mT the field was switched rapidly to 100 nT$< |\mathbf{B}_0| <$ 500 nT and three rectangular pulses of relative duration 1:2:1 were applied in the $x$, $y$ and then $x$ coils respectively. The field was then rapidly switched to 4.46 µT to detect the free precession signal after a dc $\pi/2$ pulse. A four-step phase cycle on the final dc pulse and on the receiver was used to ensure that the signal amplitude was proportional to the $z$ component of sample magnetization after the composite pulse. The resulting dependence on the pulse length is shown in Figure 3.

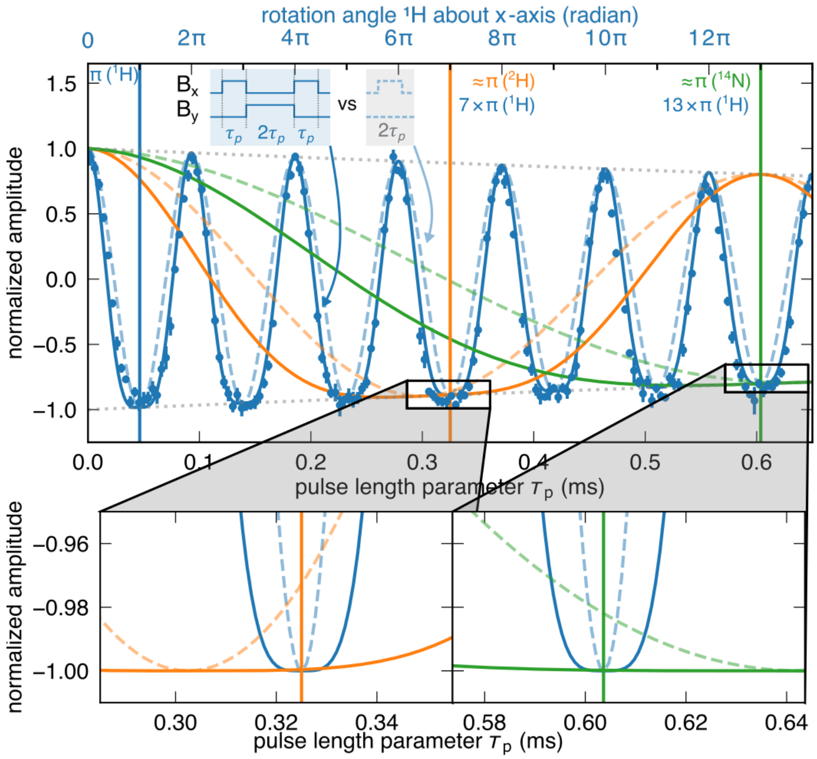


Figure 3: Experimental benchmark of composite $\pi$-pulses. Blue data points represent experimental amplitudes of $z$-magnetization after a composite $\pi$-pulse vs. duration $\tau_p$. The solid line is a fit to the analytical model $\langle I_z \rangle(\tau_p) = \cos^2(\theta)\cos(2\theta) - \sin^2(\theta)$ using $\theta = \gamma_{\rm H} B_{\rm pulse} \tau_p$ and an exponential decay to account for losses due to field inhomogeneity. For comparison, the curve $\langle I_z \rangle(\tau_p) = \cos\theta$ for a single dc-pulse is also shown (blue, dashed). Other curves plotted represent the model composite (solid) and single pulse comparison (dashed) models for $^2$H and $^{14}$N spin species; these are horizontally stretched relative to the blue curves by $\gamma_{\rm H}/\gamma_{\rm D}$ and $\gamma_{\rm H}/\gamma_{\rm 14N}$, respectively. Vertical lines at $7\pi$ (orange) and $13\pi$ (green) denote where the $\tau_p$ comes closest to an accurate $\pi$ rotation of both spin species.

The solid best-fit curve in Figure 3 confirms a wider inversion bandwidth of the composite dc pulse compared to a single dc pulse, thus widening tolerance against pulse-length errors or non-integer ratios of Rabi frequencies. The latter allows simultaneous spin flips of $^{1}$H/$^{2}$H or $^{1}$H/$^{14}$N with high fidelity. For example, as shown in the lower part of Figure 3 (orange curve), inversion maxima for $^{1}$H/$^{2}$H coincide at $\tau_p = 323$ µs with amplitudes $< -0.99$ relative to magnetization before the composite pulse, compared to $-0.97$ for a single rectangular pulse of the same duration.

## S.4 Experimental Benchmarking of XY4 Phase Cycling

Pulse fidelities were improved further by introducing the XY4 phase cycle, namely cycling the overall phase of composite pulses by 0, $\pi/2$, 0, $\pi/2$ and so on. Experimentally these were quantified in the same way as the single composite pulse by detecting an NMR signal of amplitude proportional to the $z$ magnetization, using not one but four sequential composite pulses in between the prepolarization and detection stages of the experiment. Results are shown in Figure 4. In contrast to the previous results, we are interested in the width of the regions near $\langle I_z\rangle(\tau_p)/\langle I_z\rangle(0) = +1$, the plus sign arising because an even number of $\pi$ rotations is performed.

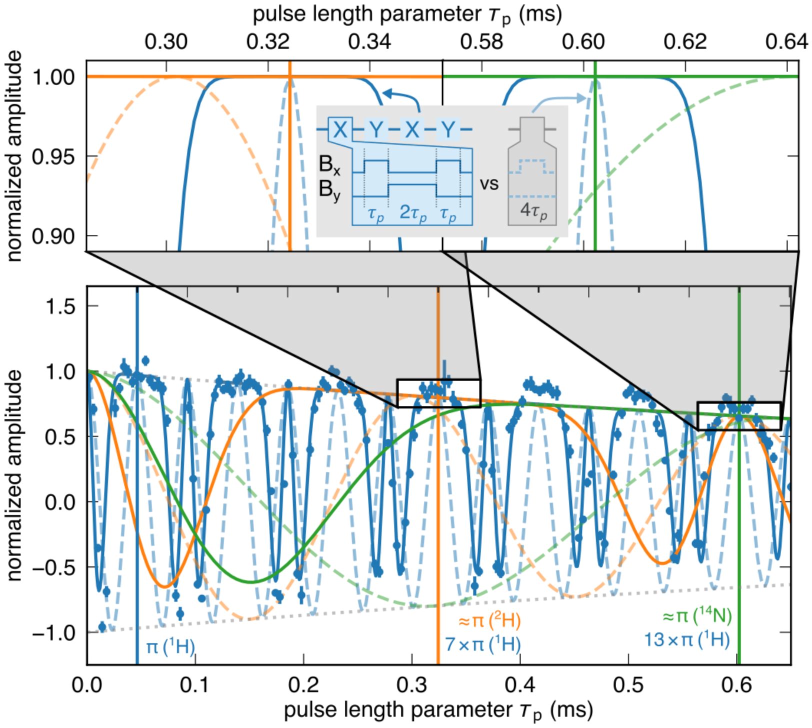


Figure 4: Experimental benchmark of XY4. Data points show amplitudes of the $z$-magnetization following four phase-cycled composite pulses (see inset), vs. $\tau_p$. The solid line gives the fit to the analytical model $\langle I_z\rangle(\tau_p)/\langle I_z\rangle(0) = [1091 - 1232\cos(2\theta) + 88\cos(4\theta) + 848\cos(6\theta) + 764\cos(8\theta) + 368\cos(10\theta) + 104\cos(12\theta) + 16\cos(14\theta) + \cos(16\theta)]/2048$ using $\theta = \gamma_{\mathrm{H}} B_{\mathrm{pulse}}\tau_p$. For comparison the theoretical performance of a single dc-pulse is shown with a dashed blue line. Orange and green curves predict behavior for $^{2}$H and $^{14}$N respectively, by horizontal stretching as described in Figure 3.

A main feature of Figure 4 is the existence of consecutive inversion maxima for $^1$H/$^2$H, occurring at $\tau_p = 230 \pm 15$ µs ($5\pi$ on $^1$H), $\tau_p = 323 \pm 20$ µs ($7\pi$ on $^1$H) and $\tau_p = 395 - 415$ µs ($9\pi$ on $^1$H). Similar coincidences for $^1$H/$^{14}$N occur around $9\pi$, $11\pi$, $13\pi$ and $15\pi$ on $^1$H, indicating that couplings involving any two of these species can in principle be selectively averaged out.

The slower exponential decay envelope around points $\langle I_z\rangle(\tau_p)/\langle I_z\rangle(0) = +1$ – in comparison to the decay envelope for Figure 3 – is attributed to additional compensation of spatial inhomogeneities in the pulsed magnetic fields by XY4.

The long-term fidelity of composite $\pi$-pulse trains in combination with XY4 phase cycling was also validated. Figure 5 shows fitted phases and amplitudes of the $\pi/2$ $^1$H precession signal in water following the sequence shown in Figure 3a of the main text. Pulse lengths $\tau_p$ were set equal to $v = 1$ (blue), $v = 7$ (orange) and $v = 13$ (green) times the $\pi/2$ dc pulse length for $^1$H, corresponding to coincident $\pi$ rotations on $^2$H or $^{14}$N.

The time between two composite $\pi$-pulses was fixed to $\tau = 10$ ms, resulting in an overall delay between prepolarization and acquisition of between $\tau = 0$ ms and $\tau = 1200$ ms. The signal amplitudes were fit to an exponential decay function $\propto \exp(-N_{\text{pulses}}\tau/T_1')$ shown by the dashed gray lines in Figure 5b, where the plotting curves all have the same time constant $T_1' = 2.0(1)$ s. These data indicate that Within experimental error the relaxation rate does not depend on $v$, and from here it is concluded that no additional decoherence is introduced by the dc pulses.

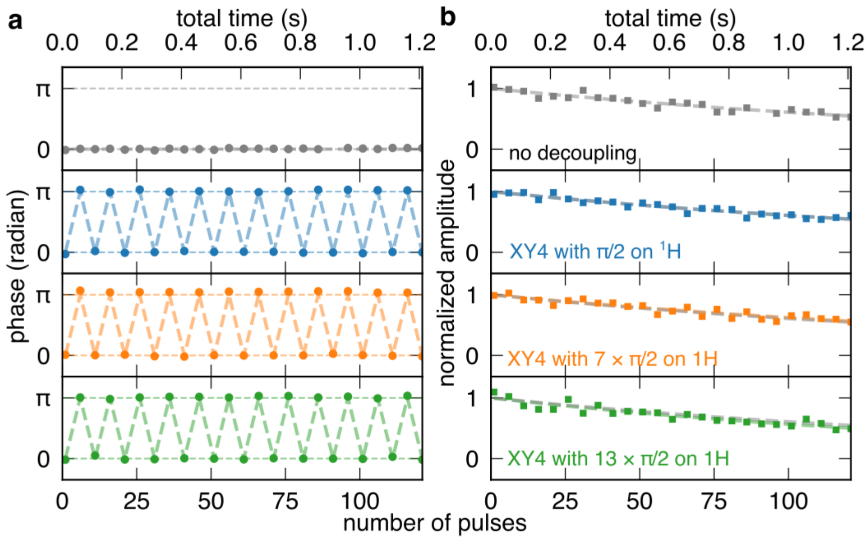


Figure 5: Phase (a) and normalized amplitude (b) of a proton precession signal subsequent to a variable number of XY4 pulses.

Finally, it is commented that the total length of the composite pulse is equal to $4\tau_{\text{p}}$, which in the longest instance for XY4($^1$H + $^{14}$N) is $\sim$2.3 ms ($v = 13$) and in the shortest case for XY4($^1$H) is $\sim$0.2 ms ($v = 1$). For an inter-pulse delay $\tau = 10$ ms these lead to pulse duty cycles of 23 % and 2 %, respectively, thus during the pulse trains the relaxation of the system remains representative of mechanisms active in ultralow field, both coherent and incoherent.

## S.5 Shimming Procedure

In the absence of decoupling pulse sequences it is challenging to impose truly zero field at the location of the NMR sample. On our experimental setup, the sample is placed in a four-layer MuMetal and ferrite shield to screen out Earth's field by a factor of $\sim 10^3$, leaving residual fields on the order of 1-10 nT. These residual fields can be partially compensated for in the $x$, $y$ and $z$ direction by applying direct current to coils located inside the shield. The compensation field along each axis is typically determined from shifts in the nuclear Larmor frequency as a function of applied compensation current during the measurement period. However, the precision of the correction field is limited by the spin relaxation time $T_2^*$.

An alternative method is through indirect probing of near-zero-field Rabi oscillations as shown in Figure 6. The amplitude of the NMR signal after switching to a high field for detection (Figure 6a) exhibits approximately monoexponential decay behavior as a function of the time delay between polarization and detection events. The decay rate is equal to the sum of the intrinsic $T_1$ relaxation rate of the sample as well as an additional, effective, contribution due to residual fields orthogonal to the polarization and detection magnetic fields. As shown in Figure 6b, the contribution of the perpendicular field is significant at $^1$H Larmor frequencies below 0.5 Hz (consistent with residual fields being on the order of 10 nT) resulting in the central or "zero-field resonance" feature seen in the plot.

Point-by-point adjustment of the perpendicular field can reduce the magnitude of the zero-field resonance feature as shown in Figure 6c. Each pixel in the two-dimensional plot represents the mean effective relaxation rate across the region $\gamma_H B_z$ between $\pm 0.5$ Hz, corresponding to the region shaded in Figure 6b; this mean should be minimized at exactly zero field. The data indicate that a best estimate of zero field is obtainable within an uncertainty of 1-2 nT. However, while precise, the procedure is extremely time consuming and must be repeated every time the magnetic shield is opened (for instance, to perform maintenance or to change the sample).

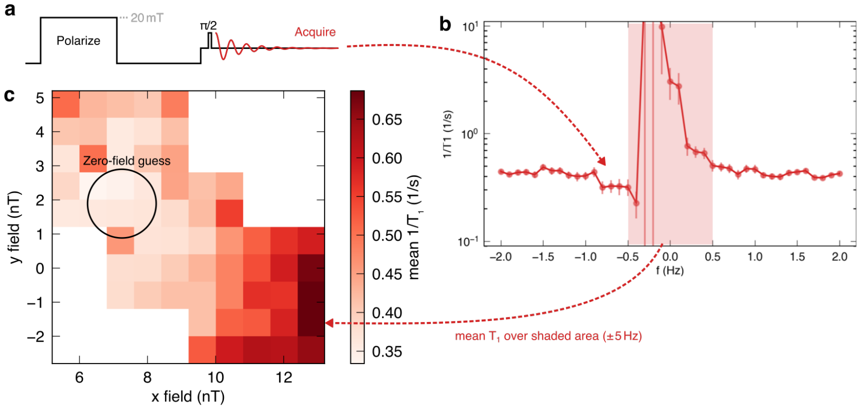


Figure 6: Zero-field shimming via effective $1/T_1$ relaxation rate. (a) fast-field-cycling pulse sequence to measure effective decay rate near zero field, for the water sample; (b) fitted monoexponential relaxation rates vs bias field along the $z$ axis; (c) variation in average relaxation rate across the central resonance feature in '(b)' vs $x$ and $y$ bias magnetic fields. The lightest-shaded pixels indicate the best estimate of zero field.

## S.6 Spin Dynamics Simulations

The following pages detail average Liouvillian theory analyses for a two-spin $I = 1/2$, $S = 1$ system. Calculations and simulations were made using Wolfram Mathematica 11.1 and the SpinDynamica package version 3.3.2.

# “Decoupling of spin decoherence paths near zero magnetic field” (Supporting information)

### This notebook is compatible with Mathematica version 11.1 and SpinDynamica version 3.3.2

In the following sections we analyze dynamics of the model two-spin system comprising one nucleus of spin quantum number I=1/2 and another of spin quantum number S=1.

Table of contents:


0. Preparation. Add SpinDynamica package to Mathematica´s filepath and define global parameters
1. Simulations of pulse-acquire 1H NMR spectra after evolution near zero field
2. Simulated evolution of the spin system’s density operator starting from Iz. Figure 3 of main paper
3. Analysis of XY4 sequences using average Hamiltonian theory (lowest order terms only)
4. Analysis of XY4 sequences using average Liouvillian theory (lowest order terms only)
5. Figure 2 of the main paper


---

## 0. Packages and definitions

### Add SpinDynamica software package to $Path. At the time of publication, version 3.3.2 can be downloaded from http://www.spindynamica.soton.ac.uk/

```
AppendTo[$Path,(* Add your path here *)];
```

```
In[2]:= Needs["SpinDynamica`"]
```

```
SpinDynamica version 3.3.2 loaded
```

### Set the spin system to spin-1/2 (I) plus spin-1 (S)
### Use gyromagnetic ratios in rad/s/microtesla

```
In[3]:= SetSpinSystem[{{"I", 1 / 2}, {"S", 1}}]
```

```
In[4]:= γH = 10^-6 GyromagneticRatio[1];
        γD = 10^-6 GyromagneticRatio[2];
        γN = 10^-6 GyromagneticRatio[14];
```

# 1. Simulations of pulse-acquire 1H NMR spectra after evolution near zero field. [I = 1H, S = Deuterium (2H)]

Here we calculate the NMR signal detected at a 1H Larmor frequency of 190 Hz after evolution under XY4 sequences near to zero field

## Spin system parameters

In[7]:=
```
γI = γH; γS = γD;
JIS = 2.5; (* intra-pair scalar coupling, in Hz *)
```

## Pulse parameters

In[9]:=
```
νpulse = 5400;(* dc pulse Rabi frequency on I spin, in Hz *)
Bpulse = 2 π νpulse / γI;
τ90pulse = 1. / (4 νpulse); (* calculate π/2 and π pulse durations, in seconds *)
τ180pulse = 2. τ90pulse;
τ = .01 ;(* evolution time in between π pulses, in seconds *)
xy4 = (π / 2) {0, 1, 0, 1}; (* phase cycle in radians *)
```

## XY4 event sequence

In[15]:=
```
cycle = xy4;
Ncycles = 300; (* arbitrary.  This is how many XY4 cycles are performed *)

ZeemanHamiltonian[Bz_] := Bz (γI opI["I", "z"] + γS opI["S", "z"]);
XY4element[v_, Bzprep_, Bpulse_] := Join @@ (((
          {ZeemanHamiltonian[Bzprep], 0} + #) & /@
        {
         {0, τ / 2},
         {Bpulse (γI opI["I", #] + γS opI["S", #]) , v τ90pulse},
         (* Composite (90X-180Y-90X)(X/Y) dc pulse *)
         {Bpulse (γI opI["I", # + π / 2] + γS opI["S", # + π / 2]) , v τ180pulse},
         {Bpulse (γI opI["I", #] + γS opI["S", #]) , v τ90pulse},
         {0, τ / 2}
        }
      ) & /@ cycle);
```

## NMR signal. We start from I-spin polarization along the z axis, allow XY4/free evolution at ultralow field, then apply a 90-degree Y pulse before detection

In[19]:=
```
signalafterXY4[Bzacq_, Bzprep_, {v_, Bpulse_}, Ncycles_] := Signal1D[{0, 4, 0.001},
   BackgroundGenerator → (ZeemanHamiltonian[Bzacq] + 2 π JIS opI["I"].opI["S"]),
   Observable → (opI["I", "x"]),
   Preparation → {Repeat[XY4element[v, (Bzprep - Bzacq), Bpulse], Ncycles],
     {RotationSuperoperator[{"I"}, {π / 2, "y"}]}},
   InitialDensityOperator → (opI["I", "z"]) (*LineBroadening→None*)];
```

## Calculate 90-acquire NMR spectrum after decoupling cycle (ν=0, ν=1 and ν=7)

In[20]:=
```
spectrumafterXY4[νIacq_, νIprep_] := Module[{},
  (* Argument 1 is the Larmor frequency oF I spin during signal acquisition, in Hz *)
  (* Argument 2 is the Larmor frequency oF I spin during preparation, in Hz *)
  {Bzacq, Bzprep} = 2 π {νIacq, νIprep} / γI; (* Convert to magnetic fields, in μT *)
  {XY4I, XY4IS, freeevolution} =
   Quiet[FT[signalafterXY4[Bzacq, Bzprep, #, 70]]] & /@ {{1, Bpulse}, {7, Bpulse}, {1, 0}};
  ListPlot[{Re[freeevolution], Re[XY4I], Re[XY4IS]},
   PlotRange → {{γI Bzacq / (2 π) - 3 JIS, γI Bzacq / (2 π) + 3 JIS}, {-1, 1} 0.05},
   FrameLabel → {"Frequency / Hz", "Re[FFT[signal]]"},
   PlotStyle → {Black, {Dashed, Red}, {Dashed, Blue}}, PlotLegends →
    {"Free evolution", "XY4(I)", "XY4(I+S)"}, AspectRatio → 0.25, ImageSize → 500]]
```

### Preparation at zero field.

Evolution under XY4(I+S) and the free Hamiltonian produce the same final spectrum

In[21]:=
```
spectrumafterXY4[190, 0.0001]
```

Out[21]=

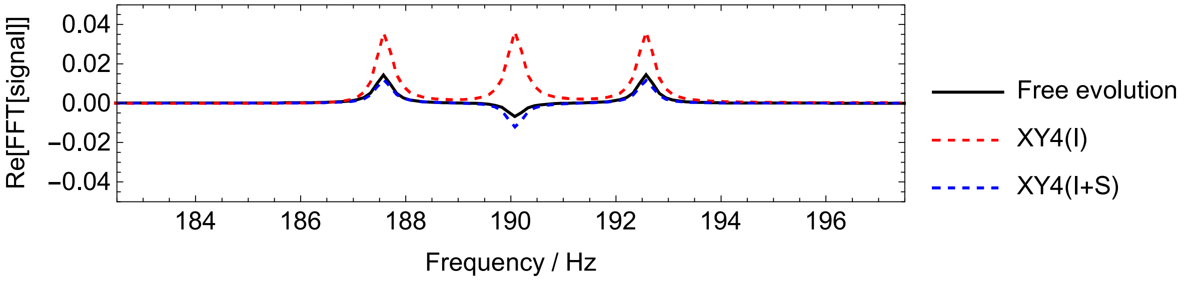


### Preparation at (practically) same field as measurement

In this "high" field limit, all sequences have same effect. Spins are decoupled by the magnetic field Bz

In[22]:=
```
spectrumafterXY4[190, 190.0001]
```

Out[22]=

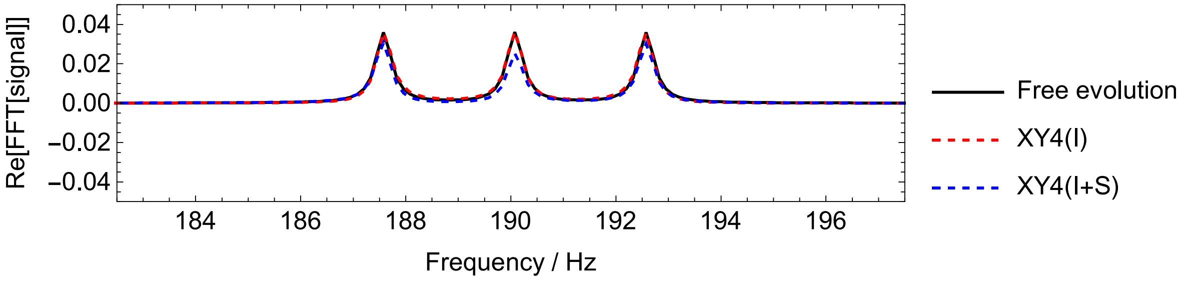


### Preparation at intermediate field

XY4 (I + S) reproduces zero-field behavior. XY4(I) produces high-field behavior, since its effect is to suppress evolution under the $J_{IS}$ coupling

In[23]:= 
```
spectrumafterXY4[190, 10]
```

Out[23]=
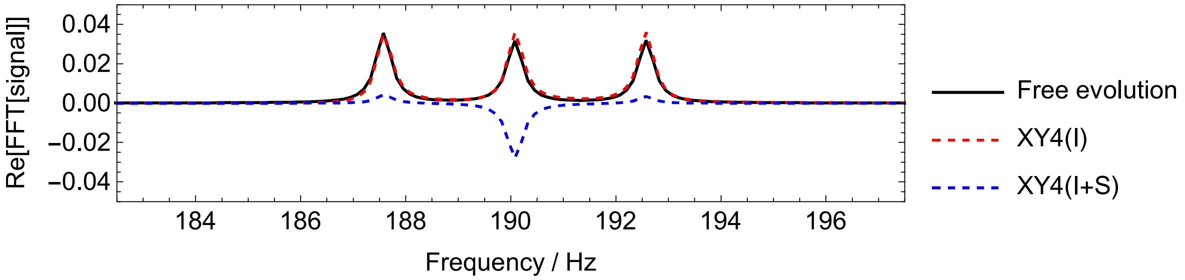


# 2. Evolution of the spin operator Iz under XY4. [I = Proton(1H), S = Deuterium (2H)]

Here we are calculating the expectation value of $I_X$, $I_Y$, $I_Z$ after every half cycle of XY4, starting from the operator $\rho(0) \propto I_Z$. We take half of the XY4 element in order to increase the time resolution of the trajectory.

In[24]:= 
```
JIS (* intra-pair scalar coupling, in Hz *)
```

Out[24]= 2.5

In[25]:= 
```
Clear[XY4element]
XY4element[v_, Bzprep_, Bpulse_] := Join @@ (((
          (* Zeeman Hamiltonian is in the background *){ZeemanHamiltonian[Bzprep], 0} + #) & /@
        {{0, τ / 2},
         {Bpulse (γI opI["I", #] + γS opI["S", #]) , v τ90pulse},
         (* Composite (90X-180Y-90X) (X/Y) dc pulse *)
         {Bpulse (γI opI["I", # + π / 2] + γS opI["S", # + π / 2]) , v τ180pulse},
         {Bpulse (γI opI["I", #] + γS opI["S", #]) , v τ90pulse},
         {0, τ / 2}}
    ) & /@ Take[cycle, 2]);
```

## Plot trajectories using same color coding as in the main text for free evolution (black), XY4(I) (red), XY4(I+S) (blue)

In[27]:= 
```
plottrajectory[κ_] := Module[{}, (* κ is the Z component
    of the dimensionless magnetic field as defined in the main text *)
   Bzprep = 2 π κ JIS / (γI - γS); (* magnetic field during preparation *);
   {trajXY4I, trajXY4IS, trajfreeevolution} = MapThread[
     TransformationAmplitudeTable[opI["I", "z"] → {opI["I", "x"], opI["I", "y"], opI["I", "z"]},
       Repeat[Evaluate[XY4element[#1, Bzprep, #2 Bpulse]], Round[2 p]], {p, 0, 60, 0.5},
       BackgroundGenerator → 2 π JIS opI["I"].opI["S"]] &, {{1, 7, 1}, {1, 1, 0}}];
   Row[MapThread[ListPlot[#1, PlotRange → {-1, 1},
       PlotStyle → {{Dashed, #2}, {Thick, Dotted, #2}, #2}, ImageSize → 400,
       PlotLegends → {"⟨Iₓ⟩" <> #3, "⟨I_Y⟩" <> #3, "⟨I_Z⟩" <> #3},
       FrameLabel → {"Number of XY4 cycles", "Operator amplitude"},
       Epilog → Inset[Framed[Style["ν_I" <> " = " <> ToString[κ] <> "×J_IS", 18],
          Background → LightYellow], {40, -0.6}]] &,
     {{trajfreeevolution, trajXY4I, trajXY4IS}, {Black, Blue, Red},
      {" free", " XY4(I)", " XY4(I+S)"}}], Spacer[50]]
  ]
```

# Plots trajectory vs dimensionless magnetic field parameter $\kappa = 2\pi \mid J_{IS} / (\gamma_I - \gamma_S) \mid$

## Zero-field / strong coupling limit

```
In[28]:= plottrajectory[0.01]
```

Out[28]=

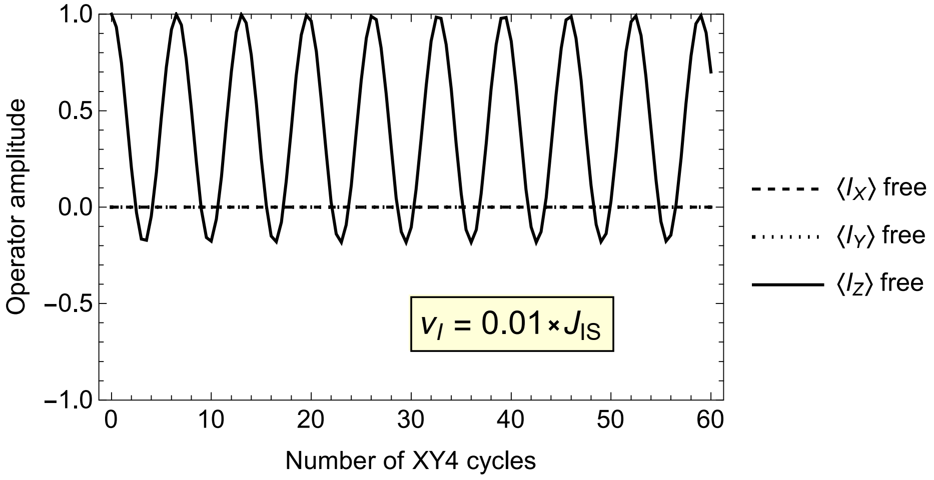


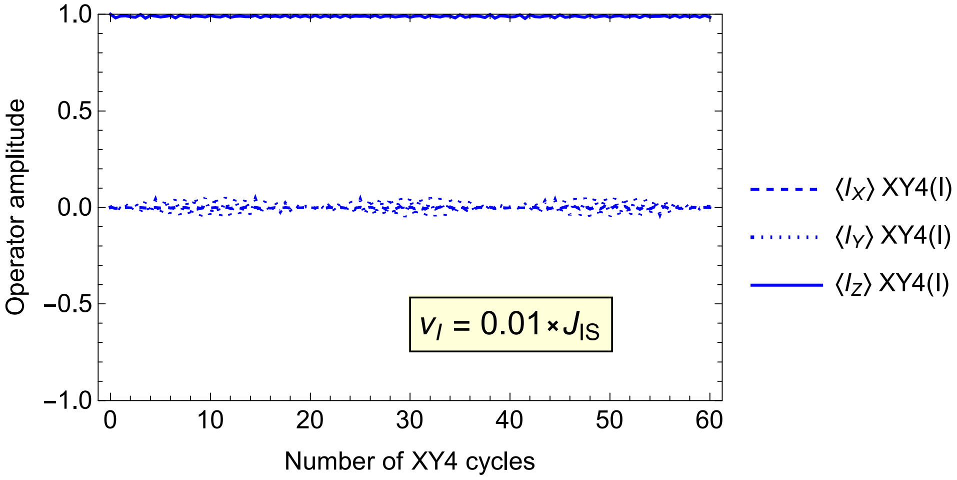


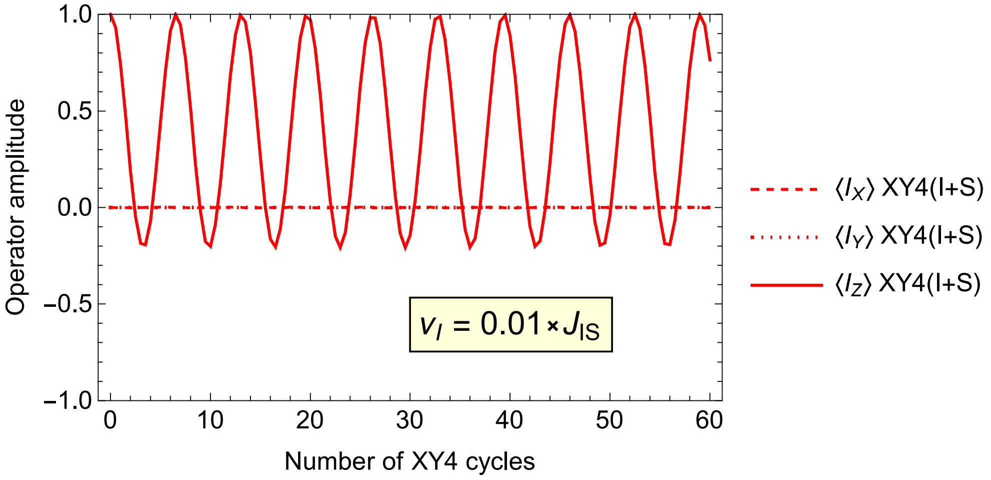

In[29]:=
```
plottrajectory[0.1]
```

Out[29]=

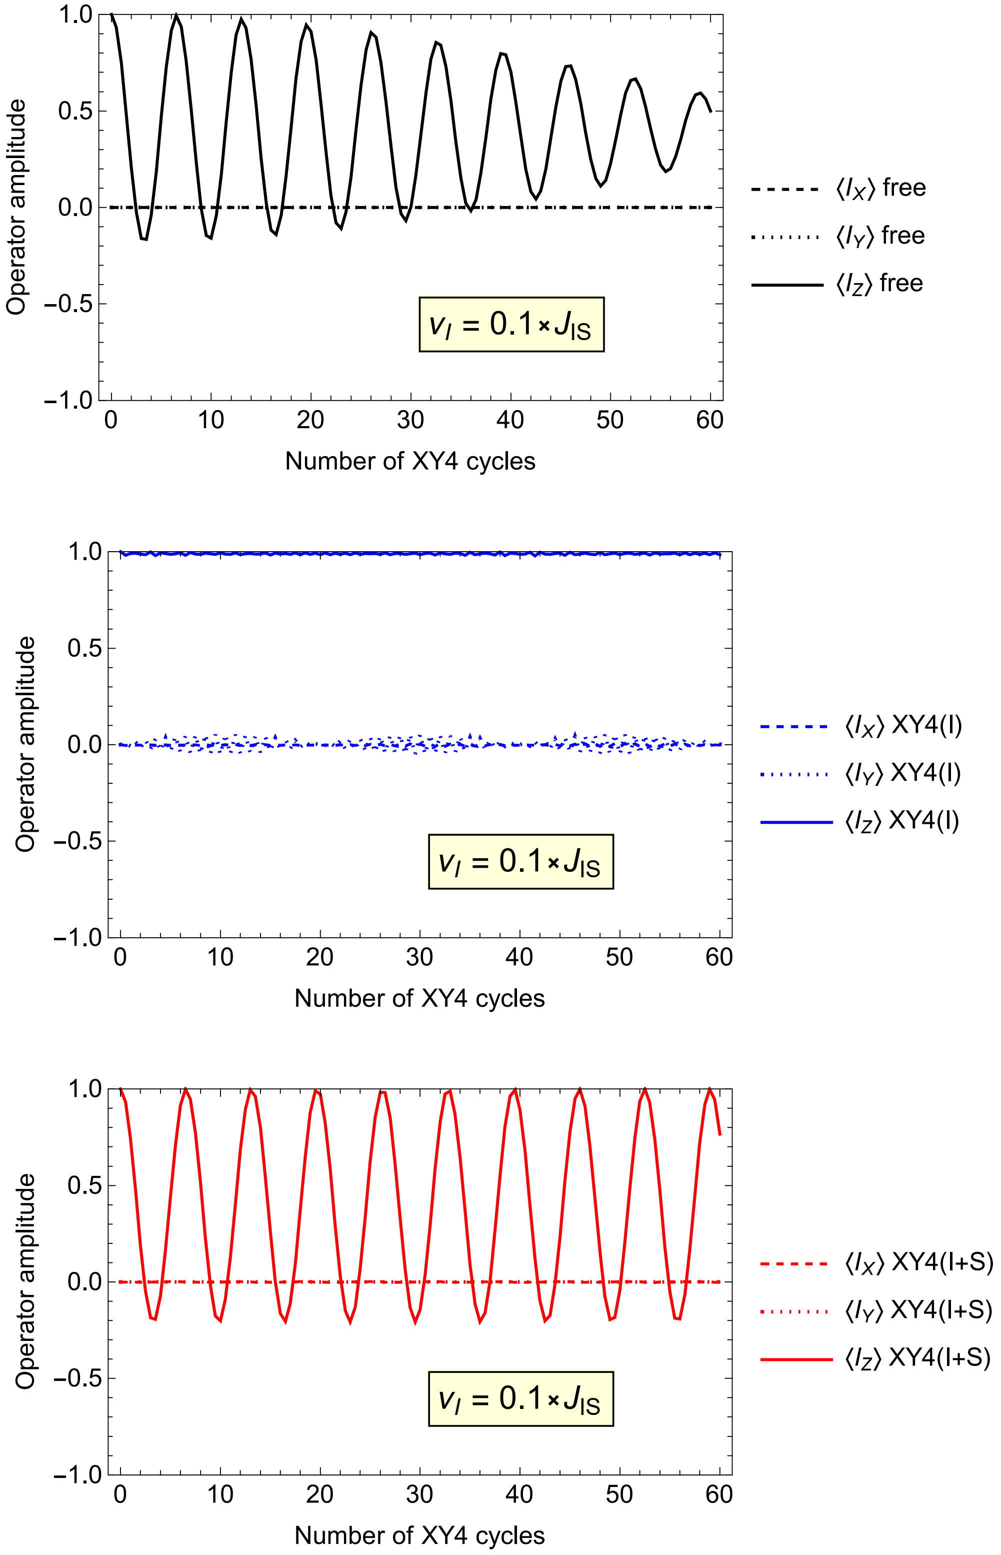

## Intermediate regime

In[30]:= `plottrajectory[0.2]`

Out[30]=

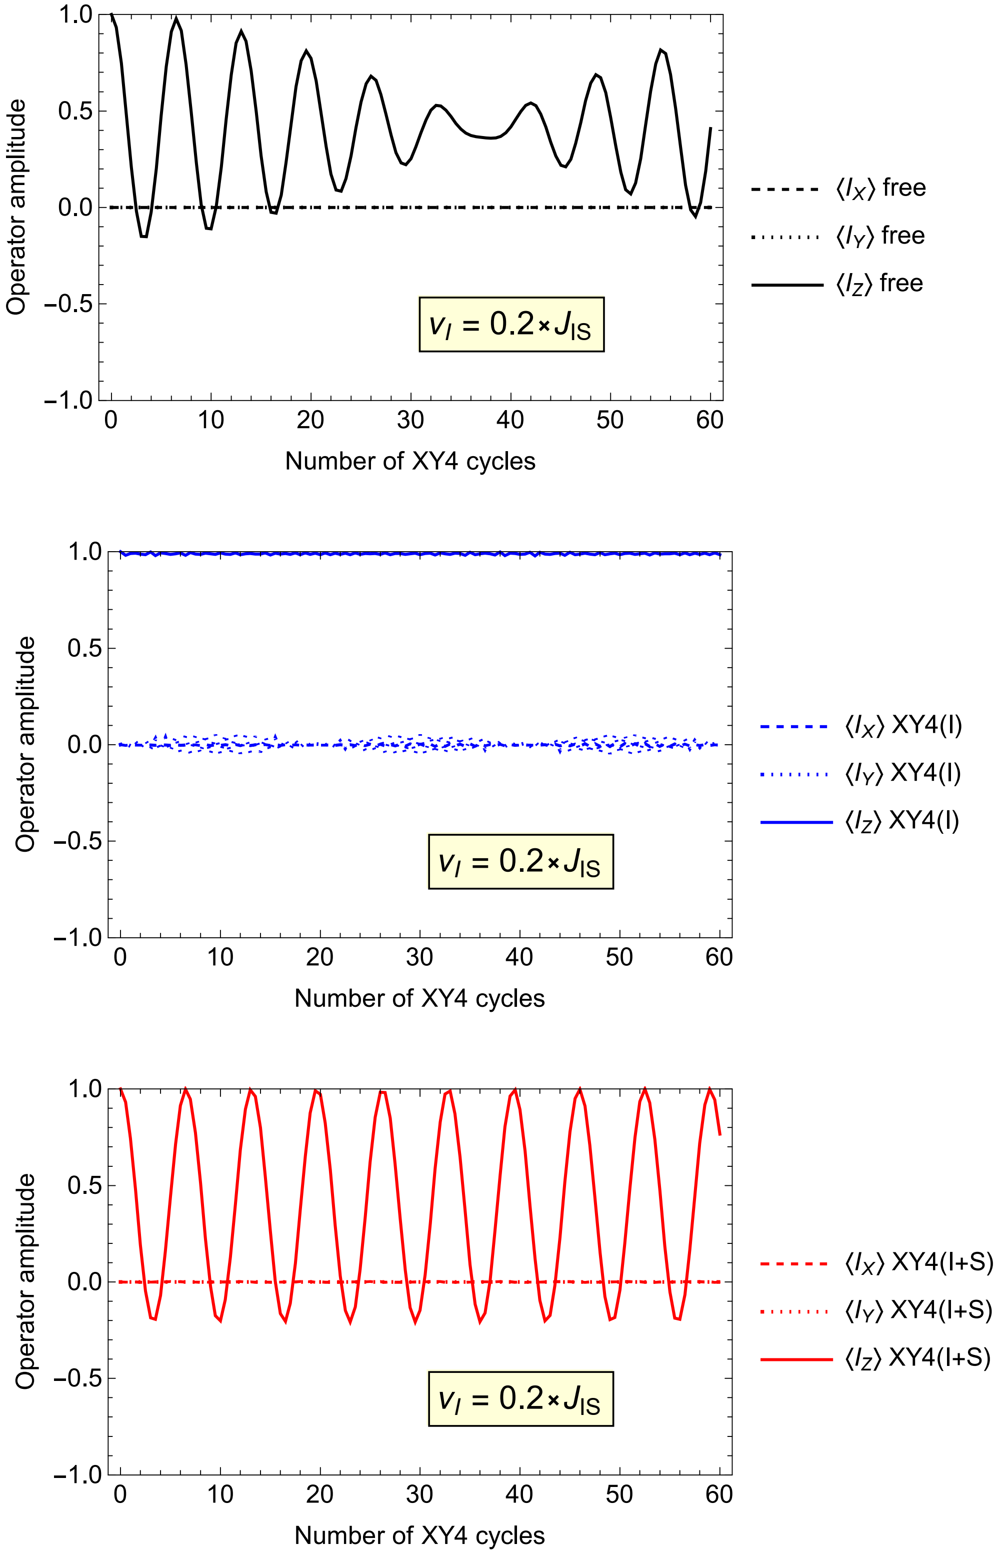

In[31]:= `plottrajectory[0.5]`

Out[31]=

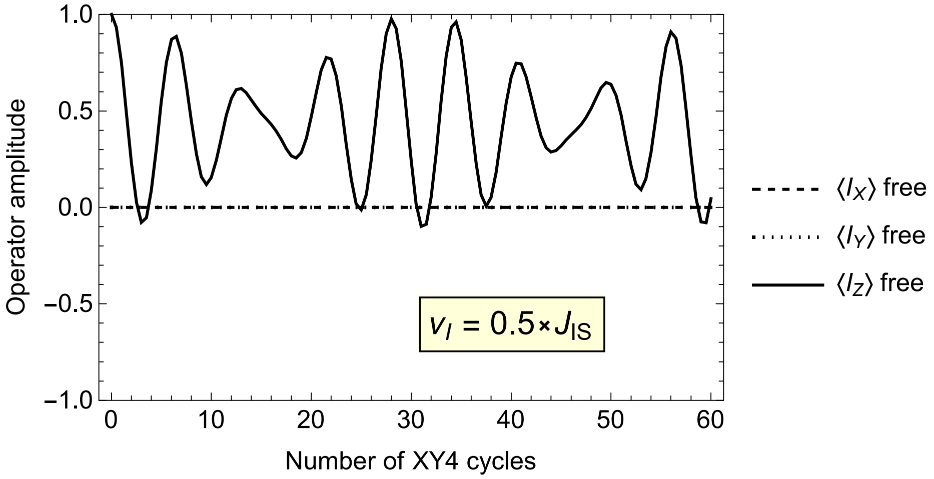


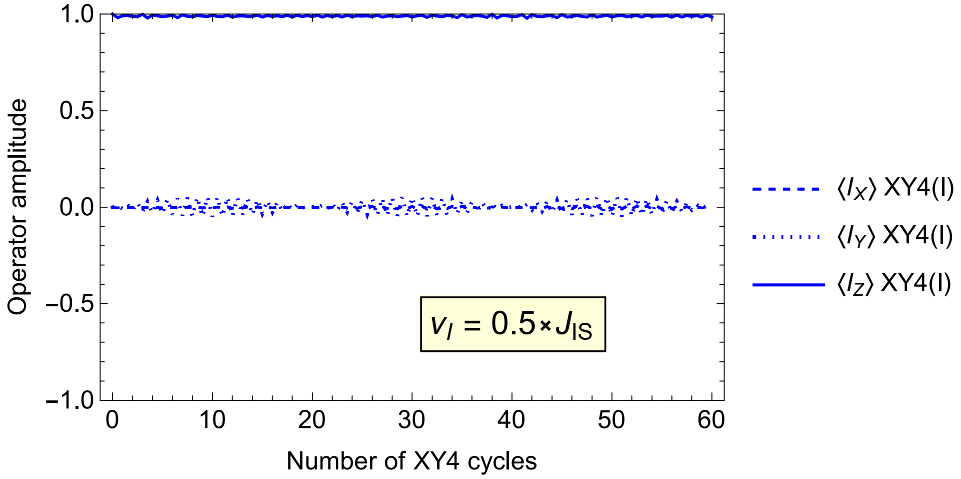


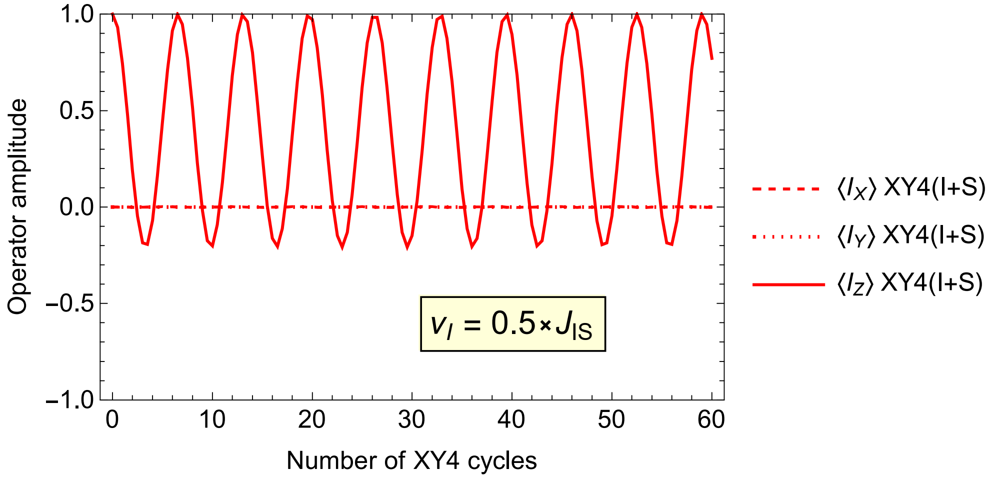

In[32]:= `plottrajectory[1]`

Out[32]=

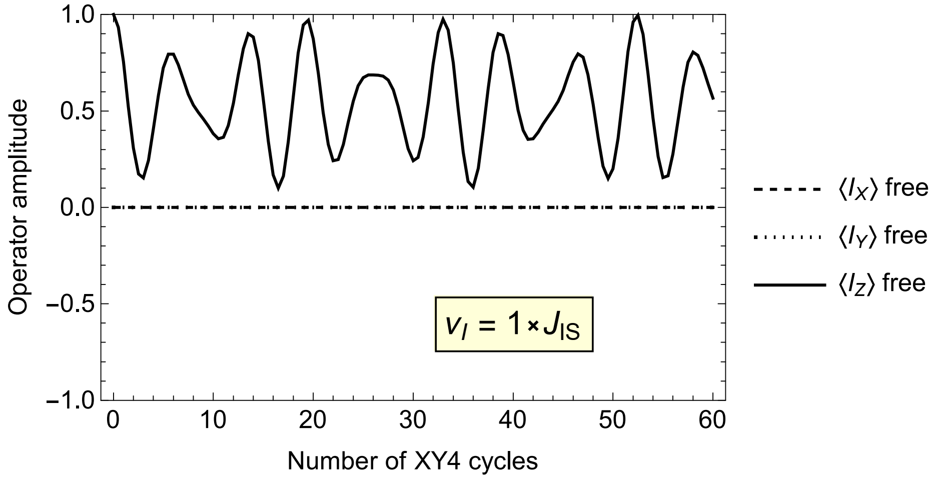


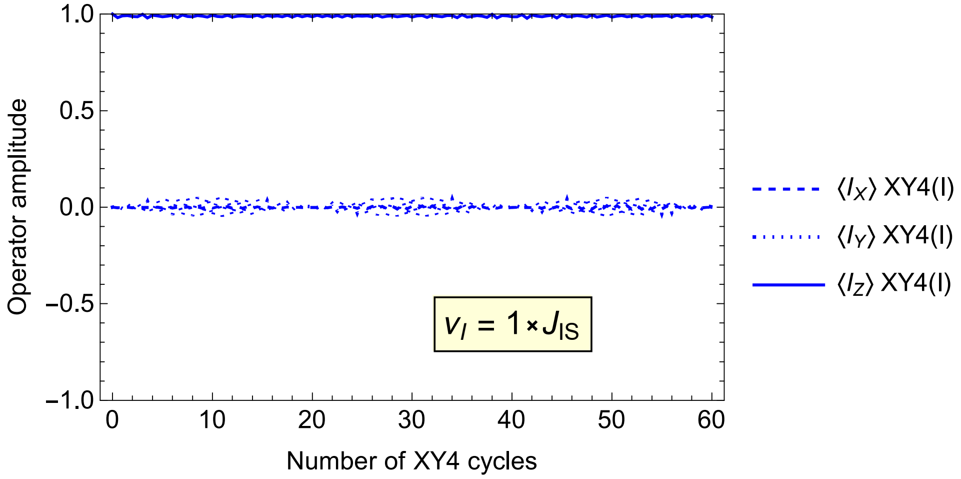


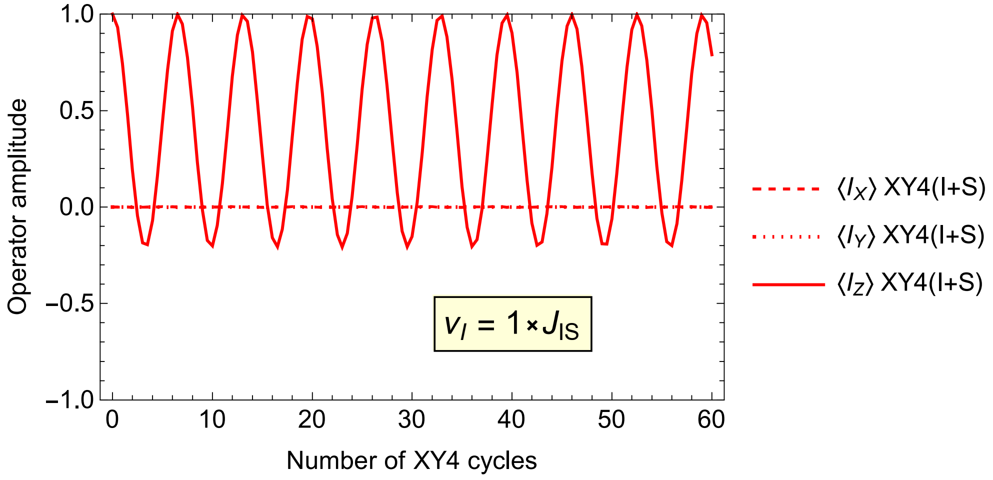

In[33]:= `plottrajectory[2]`

Out[33]=

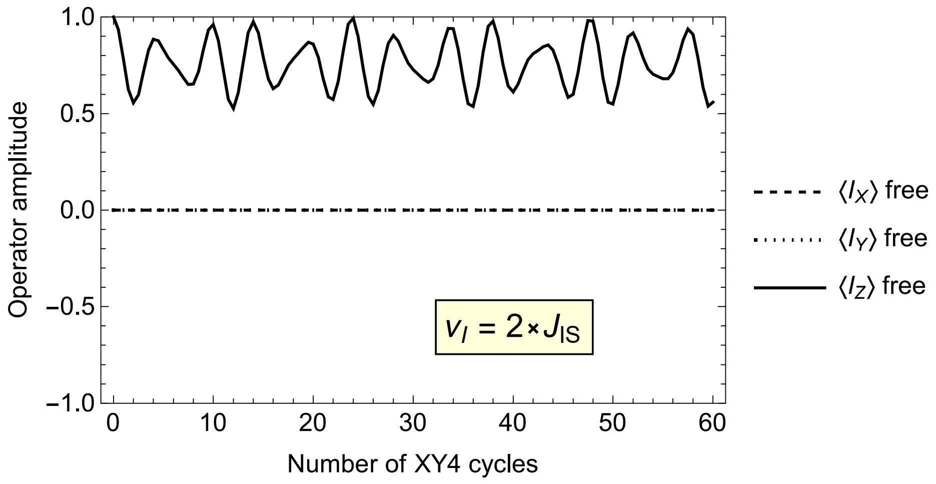


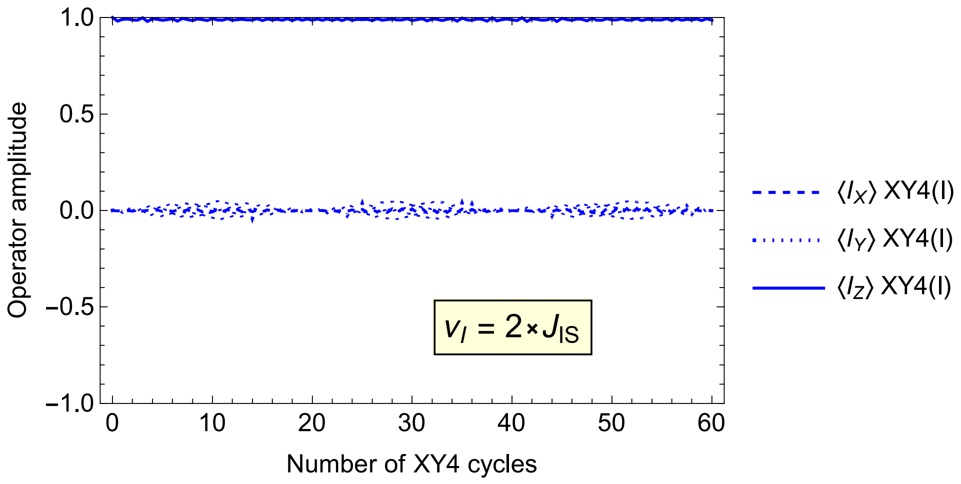


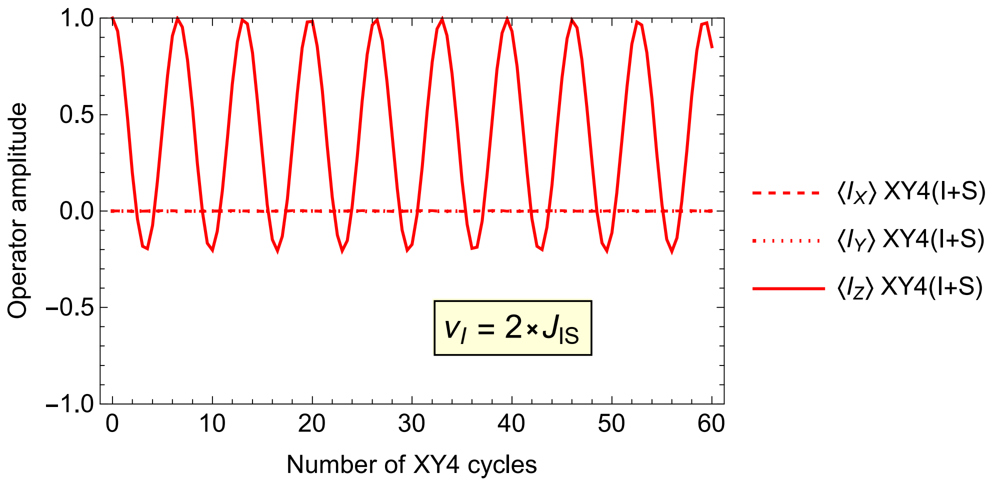

## Weak coupling limit

In[34]:= `plottrajectory[5]`

Out[34]=

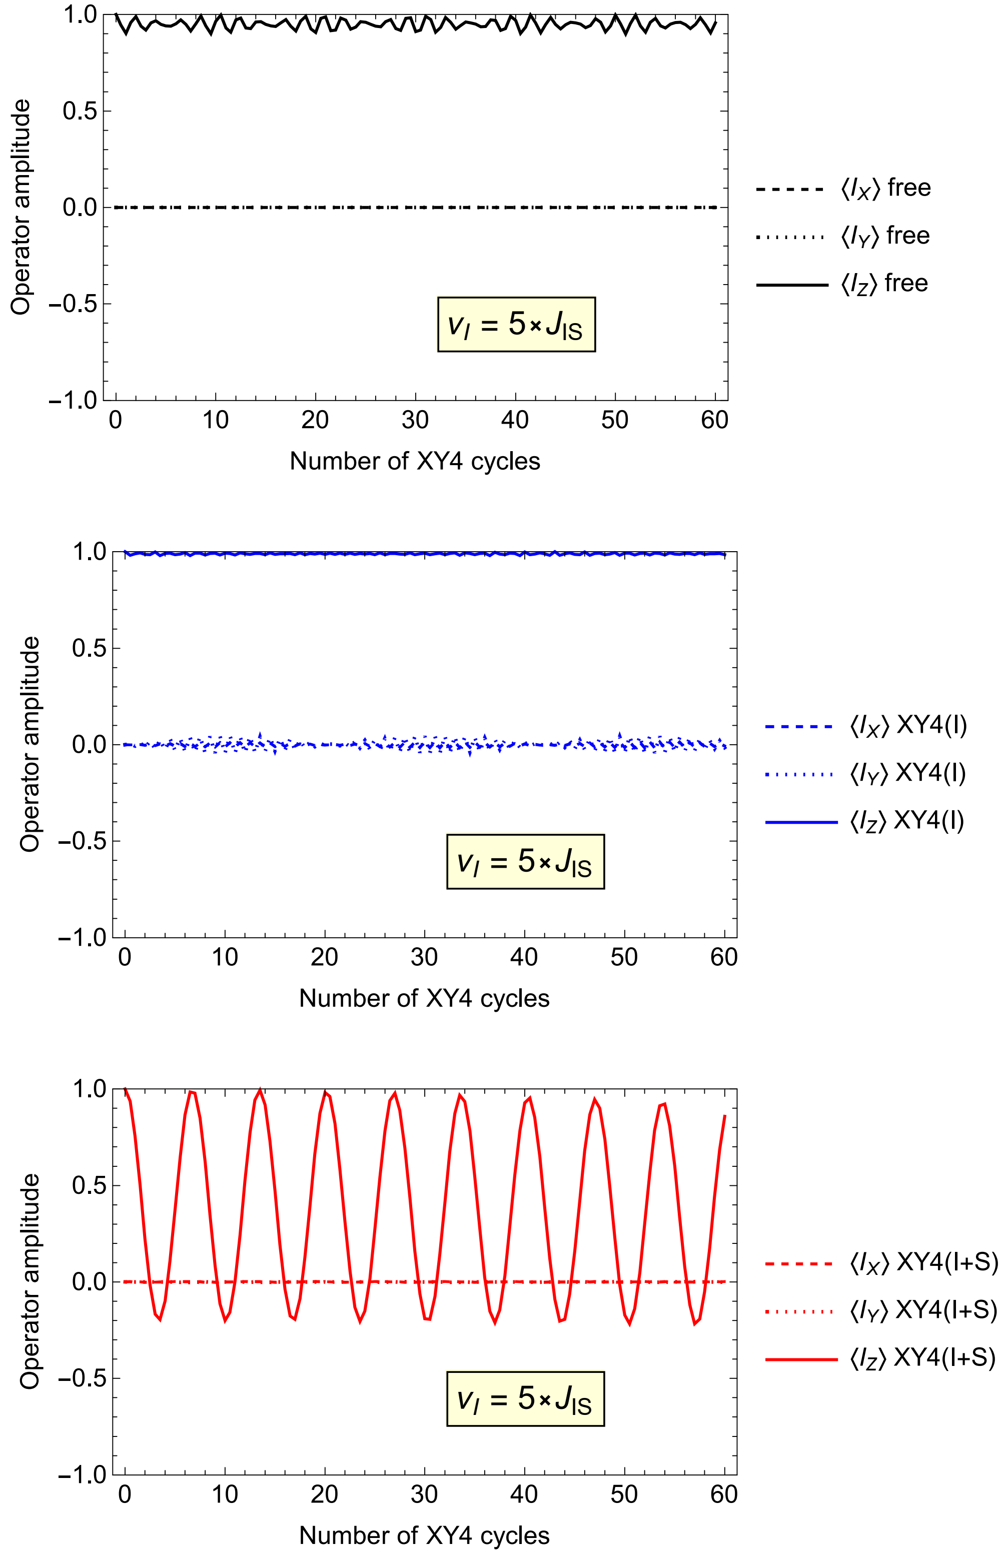

In[35]:= `plottrajectory[10]`

Out[35]=

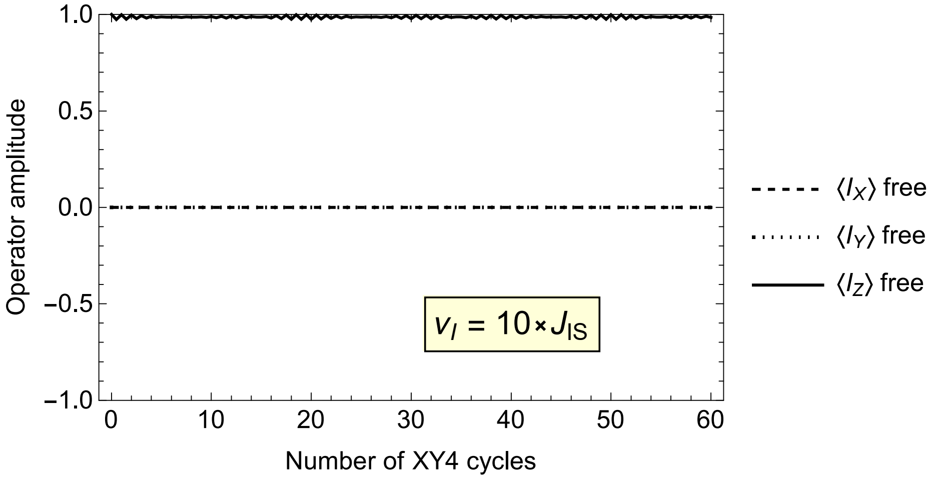


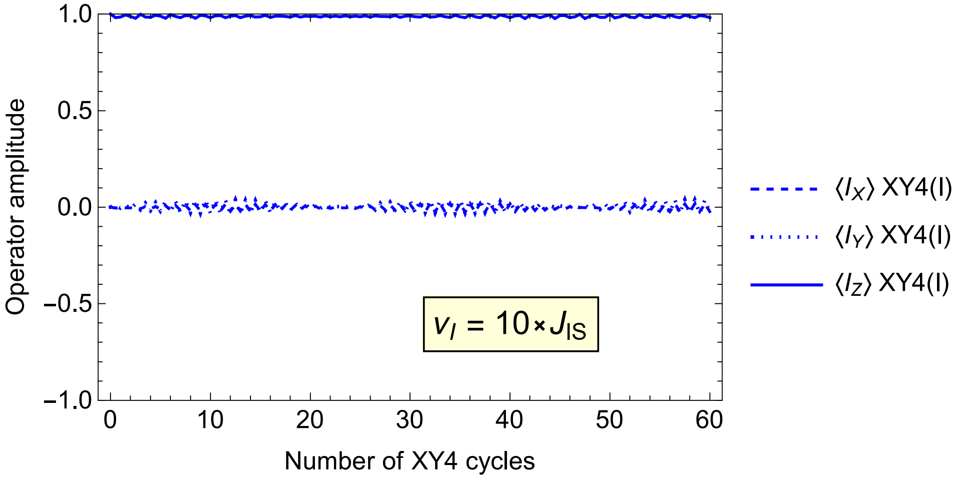


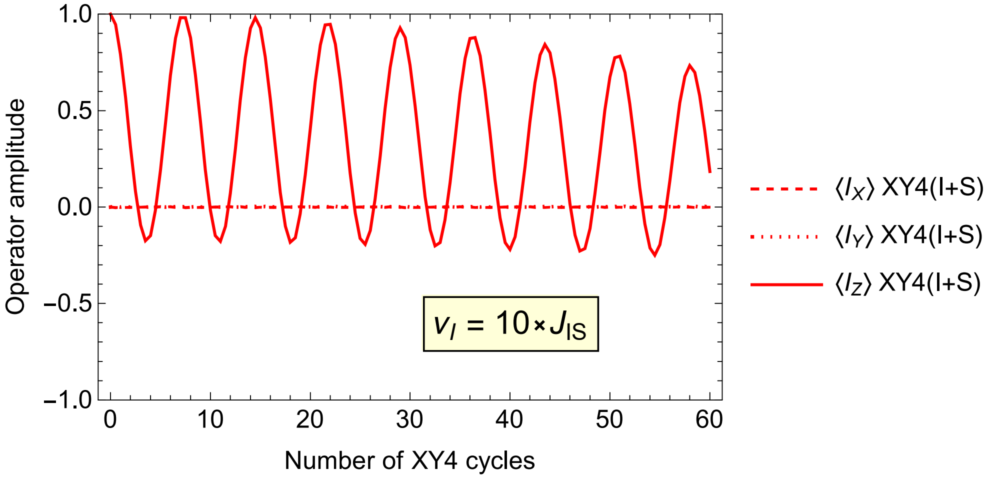

# 3. Analysis of XY4 sequences using average Hamiltonian theory (lowest order terms only)

## First, demonstrate basic averaging properties of XY4 sequences via matrix representations, assuming ideal rotation operations

### Consider rotations that act only on spin I

In[36]:=
```
? opR
```

opR[spins,angle] is the operator for rotating a single spin or a set of spins through the specified angle. If spins is absent, all spins in the current SpinSystem are rotated. The following formats for angle may be used: 1. {$\beta$,$\phi$} indicates a rotation through $\beta$ about an axis in the xy plane with the phase $\phi$. The phase value may either be numeric, or be specified using the text codes "x", "y", "–x" for the quadrature phases. A code "z" indicates a rotation about the z–axis. 2. The format {$\xi$,{$\theta$,$\phi$}} indicates a rotation through the angle $\xi$ about an axis with polar angles $\theta$ and $\phi$. 3. The format {$\alpha$,$\beta$,$\gamma$} indicates a rotation through the specified Euler angles, using the zyz convention.

In[37]:=
```
rxI = opR[{"I"}, {π, 0}] (* Rotate spin I by π radians about the x axis *)
ryI = opR[{"I"}, {π, π / 2}] (* Rotate spin S by π radians about the x axis *)
```

Out[37]= $R_{I\,x}(\pi)$

Out[38]= $R_{I\,y}(\pi)$

### Matrix representation of cumulative rotations during the XY4 element, XY4(I)

These are needed to left- and right-multiply the Hamiltonian to calculate the average Hamiltonian. We follow a similar procedure in Equation 4 of the main text, but for the average Liouvillian

In[39]:=
```
rXY4I = {rxI, rxI.ryI, rxI.ryI.rxI, rxI.ryI.rxI.ryI}
MatrixForm[Simplify[Normal[MatrixRepresentation[#]]]] & /@ rXY4I
```

Out[39]= $\{R_{I\,x}(\pi),\ R_{I\,x}(\pi)\cdot R_{I\,y}(\pi),\ R_{I\,x}(\pi)\cdot R_{I\,y}(\pi)\cdot R_{I\,x}(\pi),\ R_{I\,x}(\pi)\cdot R_{I\,y}(\pi)\cdot R_{I\,x}(\pi)\cdot R_{I\,y}(\pi)\}$

Out[40]=

$$\left\{\begin{pmatrix} 0 & -i & 0 & 0 & 0 & 0 \\ -i & 0 & 0 & 0 & 0 & 0 \\ 0 & 0 & 0 & -i & 0 & 0 \\ 0 & 0 & -i & 0 & 0 & 0 \\ 0 & 0 & 0 & 0 & 0 & -i \\ 0 & 0 & 0 & 0 & -i & 0 \end{pmatrix}, \begin{pmatrix} -i & 0 & 0 & 0 & 0 & 0 \\ 0 & i & 0 & 0 & 0 & 0 \\ 0 & 0 & -i & 0 & 0 & 0 \\ 0 & 0 & 0 & i & 0 & 0 \\ 0 & 0 & 0 & 0 & -i & 0 \\ 0 & 0 & 0 & 0 & 0 & i \end{pmatrix}, \begin{pmatrix} 0 & -1 & 0 & 0 & 0 & 0 \\ 1 & 0 & 0 & 0 & 0 & 0 \\ 0 & 0 & 0 & -1 & 0 & 0 \\ 0 & 0 & 1 & 0 & 0 & 0 \\ 0 & 0 & 0 & 0 & 0 & -1 \\ 0 & 0 & 0 & 0 & 1 & 0 \end{pmatrix}, \begin{pmatrix} -1 & 0 & 0 & 0 & 0 & 0 \\ 0 & -1 & 0 & 0 & 0 & 0 \\ 0 & 0 & -1 & 0 & 0 & 0 \\ 0 & 0 & 0 & -1 & 0 & 0 \\ 0 & 0 & 0 & 0 & -1 & 0 \\ 0 & 0 & 0 & 0 & 0 & -1 \end{pmatrix}\right\}$$

## Lowest-order average Hamiltonian for linear spin operators

In[107]:=
```
averageOperatorunderXY4element[operator_, cycle_] := Row[{operator, " ---> ",
   Mean[ExpressOperator[#.operator.Adjoint[#], CartesianProductOperatorBasis[]] & /@ cycle]}]
```

XY4 using I-spin-selective rotations has the effect of averaging all operators linear in the I spin. The S spin operators are left unperturbed

```
averageOperatorunderXY4element[opI["x"], rXY4I]
averageOperatorunderXY4element[opI["y"], rXY4I]
averageOperatorunderXY4element[opI["z"], rXY4I]
```

Out[108]= $I_x + S_x$ ---> $S_x$

Out[109]= $I_y + S_y$ ---> $S_y$

Out[110]= $I_z + S_z$ ---> $S_z$

## Lowest-order average Hamiltonian for bilinear spin operators

XY4 using I-spin-selective rotations has the effect of averaging all operators linear in the I spin

In[111]:=
```
averageOperatorunderXY4element[opI["I", "x"].opI["S", "x"], rXY4I]
averageOperatorunderXY4element[opI["I", "y"].opI["S", "y"], rXY4I]
averageOperatorunderXY4element[opI["I", "z"].opI["S", "z"], rXY4I]
```

Out[111]= $I_x \bullet S_x$ ---> 0

Out[112]= $I_y \bullet S_y$ ---> 0

Out[113]= $I_z \bullet S_z$ ---> 0

## Define rotations that act equally on both spins

In[51]:=
```
rxIS = opR[{"I", "S"}, {π, 0}] (* Rotate spin I by π radians about the x axis *)
ryIS = opR[{"I", "S"}, {π, π / 2}] (* Rotate spin S by π radians about the x axis *)
```

Out[51]= $R_{I\,x}(\pi)\bullet R_{S\,x}(\pi)$

Out[52]= $R_{I\,y}(\pi)\bullet R_{S\,y}(\pi)$

## Matrix representation of cumulative rotations during the XY4 element, both spins XY4(I+S)

In[53]:=
```
rXY4IS = {rxIS, rxIS.ryIS, rxIS.ryIS.rxIS, rxIS.ryIS.rxIS.ryIS}
MatrixForm[Simplify[Normal[MatrixRepresentation[#]]]] & /@ rXY4I
```

Out[53]= $\{R_{I\,x}(\pi)\bullet R_{S\,x}(\pi),\ R_{I\,x}(\pi)\bullet R_{I\,y}(\pi)\bullet R_{S\,x}(\pi)\bullet R_{S\,y}(\pi),\ R_{I\,x}(\pi)\bullet R_{I\,y}(\pi)\bullet R_{I\,x}(\pi)\bullet R_{S\,x}(\pi)\bullet R_{S\,y}(\pi)\bullet R_{S\,x}(\pi),$
$R_{I\,x}(\pi)\bullet R_{I\,y}(\pi)\bullet R_{I\,x}(\pi)\bullet R_{I\,y}(\pi)\bullet R_{S\,x}(\pi)\bullet R_{S\,y}(\pi)\bullet R_{S\,x}(\pi)\bullet R_{S\,y}(\pi)\}$

Out[54]=
$$\left\{\begin{pmatrix} 0 & -i & 0 & 0 & 0 & 0 \\ -i & 0 & 0 & 0 & 0 & 0 \\ 0 & 0 & 0 & -i & 0 & 0 \\ 0 & 0 & -i & 0 & 0 & 0 \\ 0 & 0 & 0 & 0 & 0 & -i \\ 0 & 0 & 0 & 0 & -i & 0 \end{pmatrix}, \begin{pmatrix} -i & 0 & 0 & 0 & 0 & 0 \\ 0 & i & 0 & 0 & 0 & 0 \\ 0 & 0 & -i & 0 & 0 & 0 \\ 0 & 0 & 0 & i & 0 & 0 \\ 0 & 0 & 0 & 0 & -i & 0 \\ 0 & 0 & 0 & 0 & 0 & i \end{pmatrix}, \begin{pmatrix} 0 & -1 & 0 & 0 & 0 & 0 \\ 1 & 0 & 0 & 0 & 0 & 0 \\ 0 & 0 & 0 & -1 & 0 & 0 \\ 0 & 0 & 1 & 0 & 0 & 0 \\ 0 & 0 & 0 & 0 & 0 & -1 \\ 0 & 0 & 0 & 0 & 1 & 0 \end{pmatrix}, \begin{pmatrix} -1 & 0 & 0 & 0 & 0 & 0 \\ 0 & -1 & 0 & 0 & 0 & 0 \\ 0 & 0 & -1 & 0 & 0 & 0 \\ 0 & 0 & 0 & -1 & 0 & 0 \\ 0 & 0 & 0 & 0 & -1 & 0 \\ 0 & 0 & 0 & 0 & 0 & -1 \end{pmatrix}\right\}$$

## Lowest-order average Hamiltonian for linear spin operators

XY4(I+S) has the effect of averaging all operators linear in the I and S spin

In[114]:=
```
averageOperatorunderXY4element[opI["x"], rXY4IS]
averageOperatorunderXY4element[opI["y"], rXY4IS]
averageOperatorunderXY4element[opI["z"], rXY4IS]
```

Out[114]= $I_x + S_x$ ---> 0

Out[115]= $I_y + S_y$ ---> 0

Out[116]= $I_z + S_z$ ---> 0

XY4(I+S) leaves unchanged all bilinear products of I and S spin operators

In[117]:=
```
averageOperatorunderXY4element[opI["I", "x"].opI["S", "x"], rXY4IS]
averageOperatorunderXY4element[opI["I", "y"].opI["S", "y"], rXY4IS]
averageOperatorunderXY4element[opI["I", "z"].opI["S", "z"], rXY4IS]
```

Out[117]= $I_x\bullet S_x$ ---> $I_x\bullet S_x$

Out[118]= $I_y\bullet S_y$ ---> $I_y\bullet S_y$

Out[119]= $I_z\bullet S_z$ ---> $I_z\bullet S_z$

# 4. Analysis of XY4 sequences using average Liouvillian theory (lowest order terms only)

## Define superoperators

### Ideal superoperators for rotations of the I spin (only)

In[65]:=
```
rxIsup = RotationSuperoperator[{"I"}, {π, 0}] ;
(* rotate spin I by π radians about the x axis *)
ryIsup = RotationSuperoperator[{"I"}, {π, π / 2}] ;
(* rotate spin I by π radians about the y axis *)
rXY4Isup = {rxIsup, rxIsup.ryIsup, rxIsup.ryIsup.rxIsup, rxIsup.ryIsup.rxIsup.ryIsup}
```

Out[67]=
```
{RotationSuperoperator[{I}, {π, x}],
 RotationSuperoperator[{I}, {π, x}].RotationSuperoperator[{I}, {π, y}],
 RotationSuperoperator[{I}, {π, x}].
  RotationSuperoperator[{I}, {π, y}].RotationSuperoperator[{I}, {π, x}],
 RotationSuperoperator[{I}, {π, x}].RotationSuperoperator[{I}, {π, y}].
  RotationSuperoperator[{I}, {π, x}].RotationSuperoperator[{I}, {π, y}]}
```

### Ideal superoperators for rotations of (both) I and S spins

In[68]:=
```
rxISsup = RotationSuperoperator[{"I", "S"}, {π, 0}] ;
(* rotate spin I by π radians about the x axis *)
ryISsup = RotationSuperoperator[{"I", "S"}, {π, π / 2}] ;
(* rotate spin I by π radians about the y axis *)
rXY4ISsup =
 {rxISsup, rxISsup.ryISsup, rxISsup.ryISsup.rxISsup, rxISsup.ryISsup.rxISsup.ryISsup}
```

Out[70]=
```
{RotationSuperoperator[{I, S}, {π, x}],
 RotationSuperoperator[{I, S}, {π, x}].RotationSuperoperator[{I, S}, {π, y}],
 RotationSuperoperator[{I, S}, {π, x}].
  RotationSuperoperator[{I, S}, {π, y}].RotationSuperoperator[{I, S}, {π, x}],
 RotationSuperoperator[{I, S}, {π, x}].RotationSuperoperator[{I, S}, {π, y}].
  RotationSuperoperator[{I, S}, {π, x}].RotationSuperoperator[{I, S}, {π, y}]}
```

### Unity superoperator for free evolution (no rotations applied)

In[71]:=
```
freeevolutionsuperoperator = {UnitySuperoperator[]}
```

Out[71]= $\{\hat{\mathbb{1}}\}$

# Define the spherical tensor operator basis

## Complete list of basis operators for the IS spin pair

In[72]:=
```
basisoperators = BasisOperators[SphericalTensorOperatorBasis[], SortBy → "CoherenceOrder"]
(* index "m" *) coherenceorders = CoherenceOrder /@ basisoperators

mesh = {1, 5, 13, 23, 31, 35}; (* coherence order *)
SetOptions[MatrixPlot, Mesh → {mesh, mesh}, ColorFunction → "Monochrome", ImageSize → 300];
```

Out[72]=

$$\Big\{\frac{1}{2}\left(I^-\cdot S^-\cdot S^-\right),\ \frac{S^-\cdot S^-}{2\sqrt{2}},\ \frac{1}{2}\left(I^-\cdot S^-\right),\ -\frac{I^-\cdot S^-\cdot S_z + I^-\cdot S_z\cdot S^- - 2\left(I_z\cdot S^-\cdot S^-\right)}{2\sqrt{3}},$$

$$\frac{I^-\cdot S^-\cdot S_z + I^-\cdot S_z\cdot S^- + I_z\cdot S^-\cdot S^-}{\sqrt{6}},\ \frac{S^-}{2\sqrt{2}},\ \frac{I^-}{\sqrt{3}},\ \frac{1}{2}\left(-\left(I^-\cdot S_z\right) + I_z\cdot S^-\right),$$

$$-\frac{I^-\cdot S_x\cdot S_x + I^-\cdot S_y\cdot S_y - 2\left(I^-\cdot S_z\cdot S_z\right) + 3\left(I^+\cdot S^-\cdot S^-\right) + 3\left(I_z\cdot S^-\cdot S_z\right) + 3\left(I_z\cdot S_z\cdot S^-\right)}{2\sqrt{15}},\ \frac{S^-\cdot S_z + S_z\cdot S^-}{2\sqrt{2}},$$

$$\frac{1}{2}\left(I^-\cdot S_z + I_z\cdot S^-\right),\ \frac{I^-\cdot S_x\cdot S_x + I^-\cdot S_y\cdot S_y - 2\left(I^-\cdot S_z\cdot S_z\right) - I^+\cdot S^-\cdot S^- + I_z\cdot S^-\cdot S_z + I_z\cdot S_z\cdot S^-}{2\sqrt{3}},$$

$$-\frac{2\left(I^-\cdot S_x\cdot S_x\right) + 2\left(I^-\cdot S_y\cdot S_y\right) - 4\left(I^-\cdot S_z\cdot S_z\right) + I^+\cdot S^-\cdot S^- - 4\left(I_z\cdot S^-\cdot S_z\right) - 4\left(I_z\cdot S_z\cdot S^-\right)}{2\sqrt{15}},$$

$$\frac{\mathbb{1}}{\sqrt{6}},\ -\frac{I^-\cdot S^+ + I^+\cdot S^- + 2\left(I_z\cdot S_z\right)}{2\sqrt{3}},\ \frac{S_z}{2},\ \sqrt{\frac{2}{3}}\,I_z,\ \frac{I^-\cdot S^+ - I^+\cdot S^-}{2\sqrt{2}},$$

$$-\frac{3\left(I^-\cdot S^+\cdot S_z\right) + 3\left(I^-\cdot S_z\cdot S^+\right) + 3\left(I^+\cdot S^-\cdot S_z\right) + 3\left(I^+\cdot S_z\cdot S^-\right) - 4\left(I_z\cdot S_x\cdot S_x\right) - 4\left(I_z\cdot S_y\cdot S_y\right) + 8\left(I_z\cdot S_z\cdot S_z\right)}{2\sqrt{30}},$$

$$-\frac{S_x\cdot S_x + S_y\cdot S_y - 2\left(S_z\cdot S_z\right)}{2\sqrt{3}},\ -\frac{I^-\cdot S^+ + I^+\cdot S^- - 4\left(I_z\cdot S_z\right)}{2\sqrt{6}},\ \frac{I^-\cdot S^+\cdot S_z + I^-\cdot S_z\cdot S^+ - I^+\cdot S^-\cdot S_z - I^+\cdot S_z\cdot S^-}{2\sqrt{2}},$$

$$-\frac{I^-\cdot S^+\cdot S_z + I^-\cdot S_z\cdot S^+ + I^+\cdot S^-\cdot S_z + I^+\cdot S_z\cdot S^- + 2\left(I_z\cdot S_x\cdot S_x\right) + 2\left(I_z\cdot S_y\cdot S_y\right) - 4\left(I_z\cdot S_z\cdot S_z\right)}{2\sqrt{5}},$$

$$-\frac{S^+}{2\sqrt{2}},\ -\frac{I^+}{\sqrt{3}},\ \frac{1}{2}\left(-\left(I^+\cdot S_z\right) + I_z\cdot S^+\right),$$

$$\frac{3\left(I^-\cdot S^+\cdot S^+\right) + I^+\cdot S_x\cdot S_x + I^+\cdot S_y\cdot S_y - 2\left(I^+\cdot S_z\cdot S_z\right) + 3\left(I_z\cdot S^+\cdot S_z\right) + 3\left(I_z\cdot S_z\cdot S^+\right)}{2\sqrt{15}},\ -\frac{S^+\cdot S_z + S_z\cdot S^+}{2\sqrt{2}},$$

$$\frac{1}{2}\left(-\left(I^+\cdot S_z\right) - I_z\cdot S^+\right),\ \frac{-\left(I^-\cdot S^+\cdot S^+\right) + I^+\cdot S_x\cdot S_x + I^+\cdot S_y\cdot S_y - 2\left(I^+\cdot S_z\cdot S_z\right) + I_z\cdot S^+\cdot S_z + I_z\cdot S_z\cdot S^+}{2\sqrt{3}},$$

$$\frac{I^-\cdot S^+\cdot S^+ + 2\left(I^+\cdot S_x\cdot S_x + I^+\cdot S_y\cdot S_y - 2\left(I^+\cdot S_z\cdot S_z + I_z\cdot S^+\cdot S_z + I_z\cdot S_z\cdot S^+\right)\right)}{2\sqrt{15}},\ \frac{S^+\cdot S^+}{2\sqrt{2}},\ \frac{1}{2}\left(I^+\cdot S^+\right),$$

$$\frac{I^+\cdot S^+\cdot S_z + I^+\cdot S_z\cdot S^+ - 2\left(I_z\cdot S^+\cdot S^+\right)}{2\sqrt{3}},\ \frac{I^+\cdot S^+\cdot S_z + I^+\cdot S_z\cdot S^+ + I_z\cdot S^+\cdot S^+}{\sqrt{6}},\ -\frac{1}{2}\left(I^+\cdot S^+\cdot S^+\right)\Big\}$$

Out[73]=

{-3, -2, -2, -2, -2, -1, -1, -1, -1, -1, -1, -1, -1,
0, 0, 0, 0, 0, 0, 0, 0, 0, 0, 1, 1, 1, 1, 1, 1, 1, 1, 2, 2, 2, 2, 3}

## Selected basis operators, for reference purposes

In[76]:=
```
(* Identity, Iz and Sz *)
basisoperators[[#]] & /@ {14, 16, 17}
```

Out[76]= $\left\{\frac{\mathbb{1}}{\sqrt{6}}, \frac{S_z}{2}, \sqrt{\frac{2}{3}}\ I_z\right\}$

## Calculate matrix representation of the XY4-averaged Liouvillian superoperator ($L^{(0)}$ term only)

For coherent evolution, we use the following function

```
In[77]:= averageLiouvillianunderXY4element[Liouvillian_, cycle_] := (1 / Length[cycle]) Plus @@ (
      SuperoperatorMatrixRepresentation[#, SphericalTensorOperatorBasis[]].
         SuperoperatorMatrixRepresentation[Liouvillian, SphericalTensorOperatorBasis[]].
         Adjoint[SuperoperatorMatrixRepresentation[#, SphericalTensorOperatorBasis[]]] & /@
       cycle)
```

and for plotting...

```
In[78]:= plotAverageLiouvillianSuperoperatorMatrixRepresentation[Liouvillian_, cycle_] := MatrixPlot[
    Simplify[Normal[averageLiouvillianunderXY4element[Liouvillian, cycle]]], ImageSize → 250]
```

## Application to each term of Equation 1

## I-S scalar coupling ($J_{IS}$)

free evolution --> no averaging

In[79]:=
```
Jfree = plotAverageLiouvillianSuperoperatorMatrixRepresentation[
  -I CommutationSuperoperator["JIS" opI["I"].opI["S"]], freeevolutionsuperoperator]
```

Out[79]=

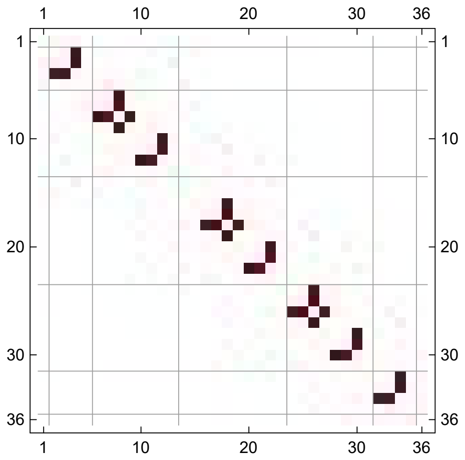


XY4(I) --> complete averaging

In[80]:=
```
JXY4I = plotAverageLiouvillianSuperoperatorMatrixRepresentation[
  -I CommutationSuperoperator["JIS" opI["I"].opI["S"]], rXY4Isup]
```

Out[80]=

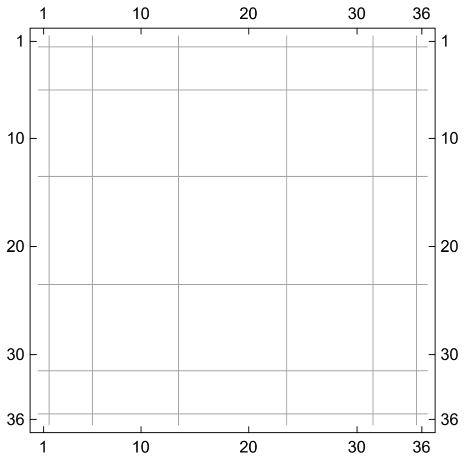


XY4(I+S) --> no averaging

In[81]:=
```
JXY4IS = plotAverageLiouvillianSuperoperatorMatrixRepresentation[
  -I CommutationSuperoperator["JIS" opI["I"].opI["S"]], rXY4ISsup]
```

Out[81]=

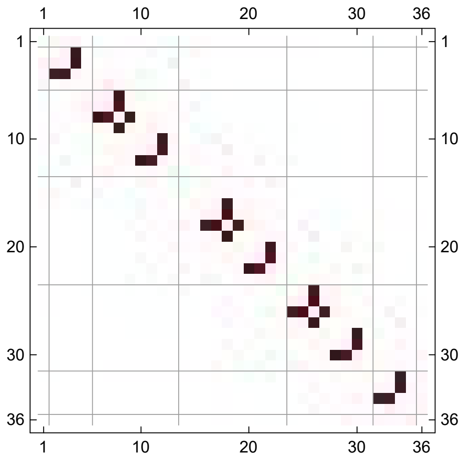

## Zeeman interaction, I spin

free evolution --> no averaging

In[82]:=
```
ZIfree = plotAverageLiouvillianSuperoperatorMatrixRepresentation[
  -I CommutationSuperoperator["γI" opI["I"].{Bx0, By0, Bz0}], freeevolutionsuperoperator]
```

Out[82]=
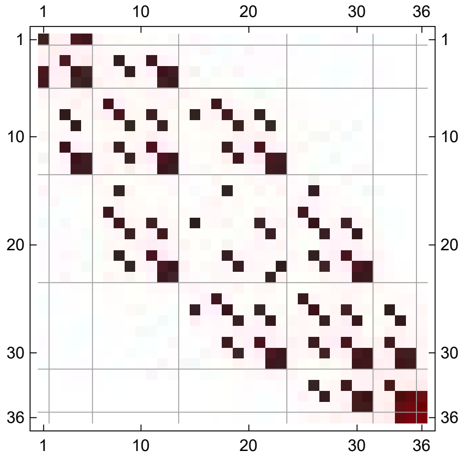


XY4(I) --> complete averaging

In[83]:=
```
ZIXY4I = plotAverageLiouvillianSuperoperatorMatrixRepresentation[
  -I CommutationSuperoperator["γI" opI["I"].{Bx0, By0, Bz0}], rXY4Isup]
```

Out[83]=
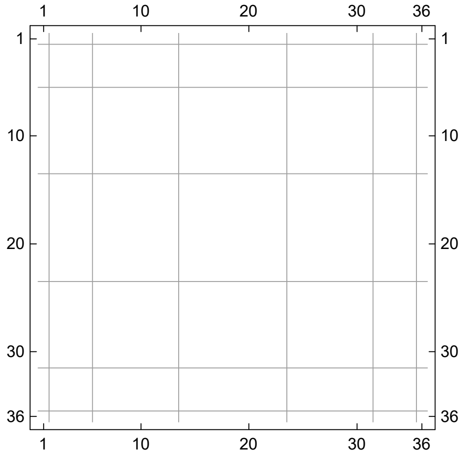


XY4(I+S) --> complete averaging

In[84]:=
```
ZIXY4IS = plotAverageLiouvillianSuperoperatorMatrixRepresentation[
  -I CommutationSuperoperator["γI" opI["I"].{Bx0, By0, Bz0}], rXY4ISsup]
```

Out[84]=
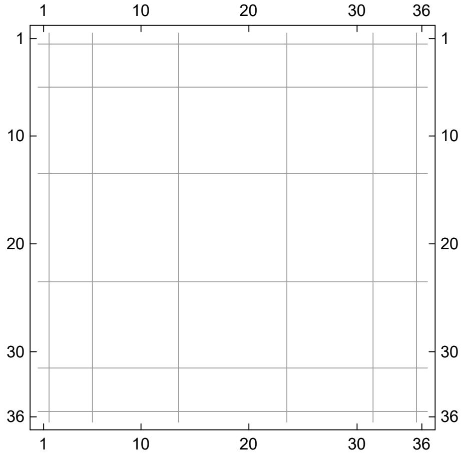

## Zeeman interaction, S spin

free evolution --> no averaging

In[85]:=
```
ZSfree = plotAverageLiouvillianSuperoperatorMatrixRepresentation[
  -I CommutationSuperoperator["γS" opI["S"].{Bx0, By0, Bz0}], freeevolutionsuperoperator]
```

Out[85]=

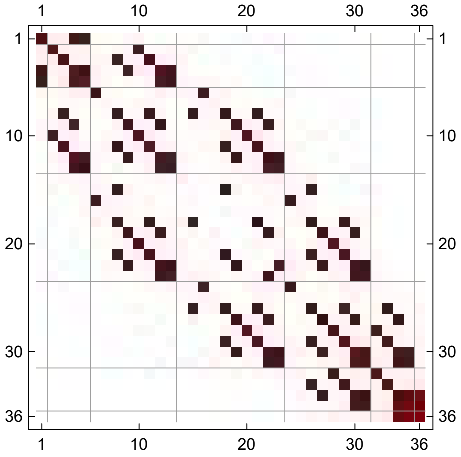


XY4(I) --> no averaging

In[86]:=
```
ZSXY4I = plotAverageLiouvillianSuperoperatorMatrixRepresentation[
  -I CommutationSuperoperator["γS" opI["S"].{Bx0, By0, Bz0}], rXY4Isup]
```

Out[86]=

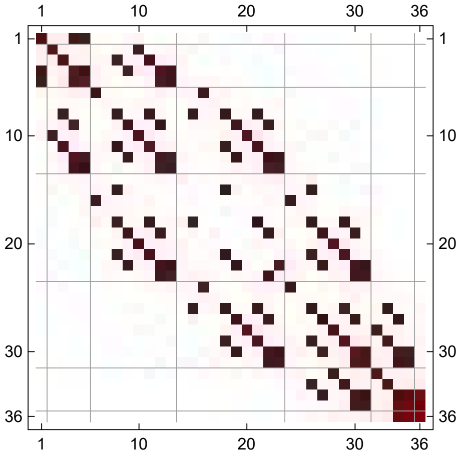


XY4(I+S) --> complete averaging

In[87]:=
```
ZSXY4IS = plotAverageLiouvillianSuperoperatorMatrixRepresentation[
  -I CommutationSuperoperator["γS" opI["S"].{Bx0, By0, Bz0}], rXY4ISsup]
```

Out[87]=

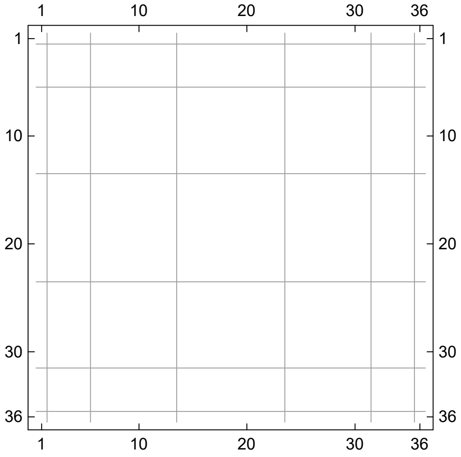

## Matrix representation of average Liouvillian superoperator: contribution from dipole-dipole relaxation and cross-correlated random field relaxation

In[88]:=
```
opR[{π, "x"}]
```

Out[88]= $R_{I\,x}(\pi)\bullet R_{S\,x}(\pi)$

In[89]:=
```
opT[{"I", "S"}, {2, -1}, 1]
```

Out[89]= $\frac{1}{2}\left(I^{-}\bullet S_z + I_z\bullet S^{-}\right)$

N.B. Superoperator is divided by the usual factor "$A^2\tau_C$"

In[90]:=
```
averageDipoleDipoleRelaxationSuperoperatorMatrixRepresentation[cycle_] :=
  1/Length[cycle] Plus @@
   (SuperoperatorMatrixRepresentation[6/5 Sum[(-1)^m DoubleCommutationSuperoperator[#.opT[
          {"I", "S"}, {2, m}, 1].Adjoint[#], #.opT[{"I", "S"}, {2, -m}, 1].Adjoint[#]],
        {m, -2, 2}], SphericalTensorOperatorBasis[]] & /@ cycle)
```

In[91]:=
```
plotAverageDipoleDipoleRelaxationSuperoperatorMatrixRepresentation[cycle_] := MatrixPlot[
  Simplify[Normal[averageDipoleDipoleRelaxationSuperoperatorMatrixRepresentation[cycle]]],
  ImageSize → 250]
```

Free evolution: DD relaxation superoperator is block-diagonal in coherence order and spherical tensor rank

In[92]:=
```
Γddfree = plotAverageDipoleDipoleRelaxationSuperoperatorMatrixRepresentation[{opR[{0, "x"}]}]
```

Out[92]=

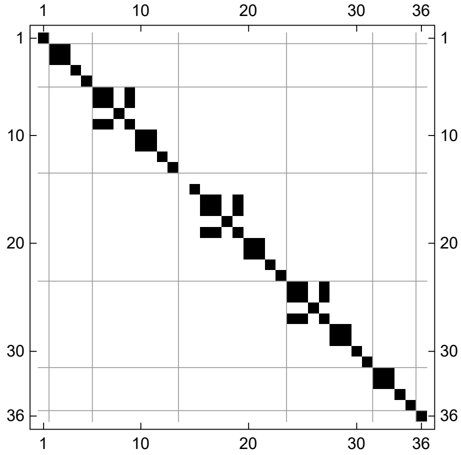


XY4(I) --> partial averaging of the central m=0 -> m'=0 block

In[93]:=
```
ΓddXY4I = plotAverageDipoleDipoleRelaxationSuperoperatorMatrixRepresentation[rXY4I]
```

Out[93]=

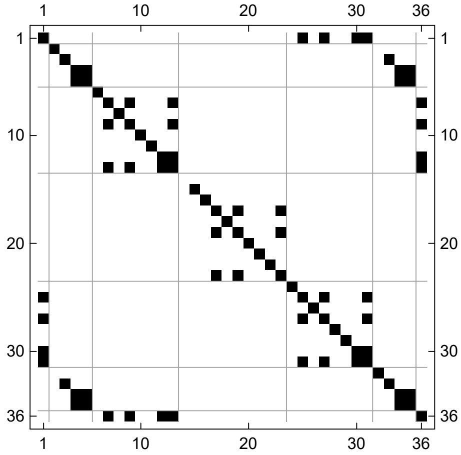


XY4(I+S) --> same as free evolution

In[94]:=
```
ΓddXY4IS = plotAverageDipoleDipoleRelaxationSuperoperatorMatrixRepresentation[rXY4IS]
```

Out[94]=

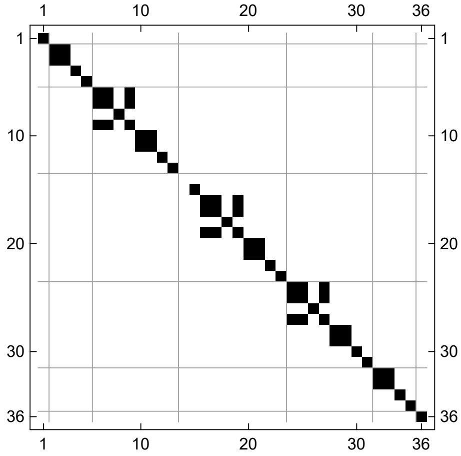

In[95]:=
```
averageRandomFieldCrossCorrelatedRelaxationSuperoperatorMatrixRepresentation[cycle_] :=
  1/Length[cycle]
   Plus @@ (SuperoperatorMatrixRepresentation[1/3 Sum[(-1)^m DoubleCommutationSuperoperator[
          #.opT[{"I"}, {1, m}].Adjoint[#], #.opT[{"S"}, {1, -m}].Adjoint[#]],
         {m, -1, 1}], SphericalTensorOperatorBasis[]] & /@ cycle)
```

In[96]:=
```
plotaverageRandomFieldCrossCorrelatedRelaxationSuperoperatorMatrixRepresentation[cycle_] :=
  MatrixPlot[Simplify[
    Normal[averageRandomFieldCrossCorrelatedRelaxationSuperoperatorMatrixRepresentation[
      cycle]]], ImageSize → 250]
```

Free evolution: DD relaxation superoperator is block-diagonal in coherence order and spherical tensor rank

In[97]:=
```
Γrffree = plotaverageRandomFieldCrossCorrelatedRelaxationSuperoperatorMatrixRepresentation[
  {opR[{0, "x"}]}]
```

Out[97]=

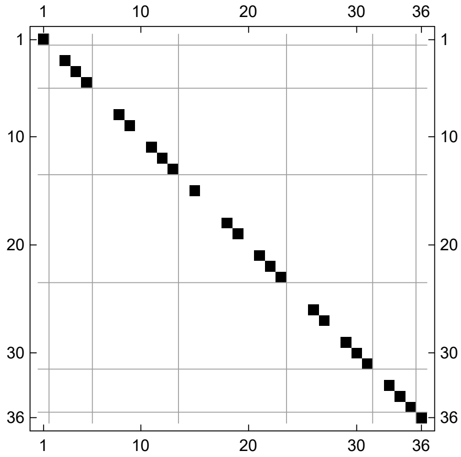


XY4(I) --> complete averaging of the cross-correlation term

In[98]:=
```
ΓrfXY4I =
 plotaverageRandomFieldCrossCorrelatedRelaxationSuperoperatorMatrixRepresentation[rXY4I]
```

Out[98]=

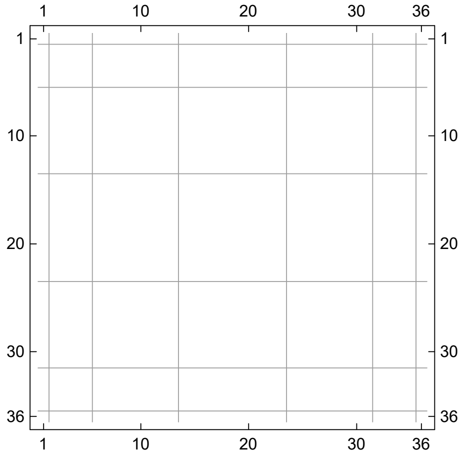


XY4(I+S) --> same as free evolution

In[99]:=
```
ΓrfXY4IS =
 plotaverageRandomFieldCrossCorrelatedRelaxationSuperoperatorMatrixRepresentation[rXY4IS]
```

Out[99]=

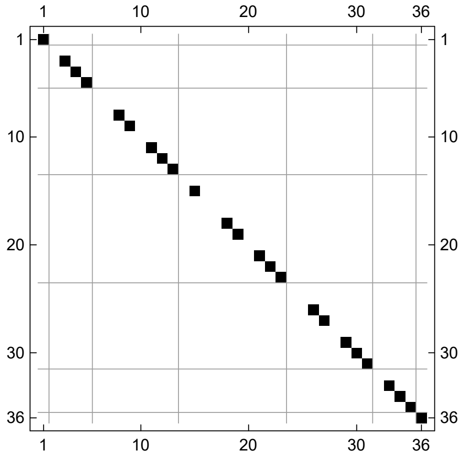

# 5. Collect together all contributions to $L^{(0)}$ from section 4.

These matrices are presented in Figure 2 of the main paper.

```
Figure2 = {
   {Jfree, ZIfree, ZSfree, Γddfree, Γrffree},
   {JXY4I, ZIXY4I, ZSXY4I, ΓddXY4I, ΓrfXY4I},
   {JXY4IS, ZIXY4IS, ZSXY4IS, ΓddXY4IS, ΓrfXY4IS}
  } // TableForm
```

Out[127]//TableForm=

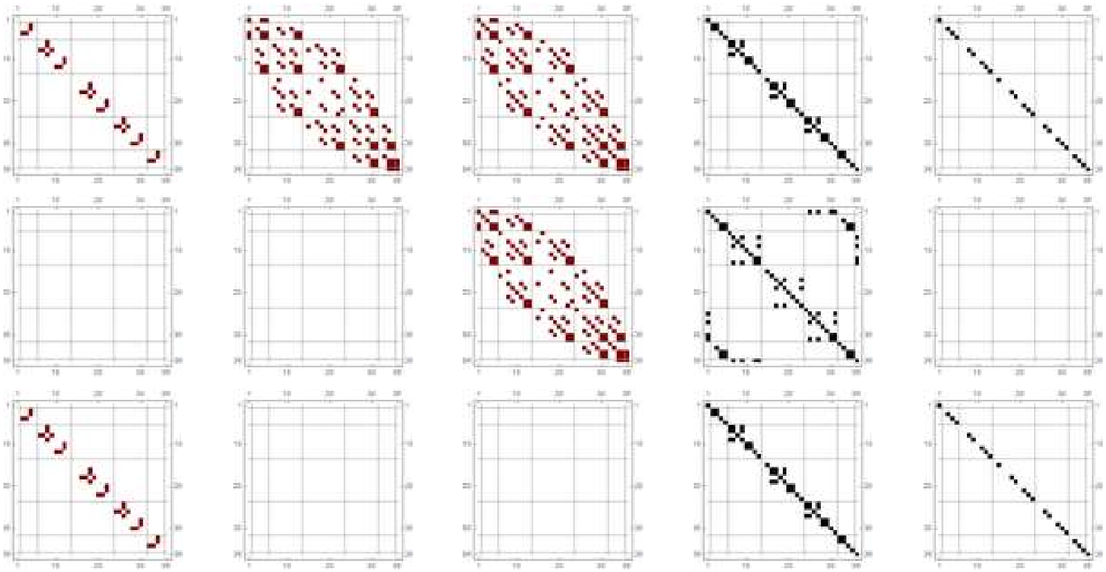

# Analytical expressions for the matrix elements can also be examined

## For example, this is the zero-quantum block of $L^{(0)}$ for the J coupling interaction

In[120]:=
```
Take[basisoperators, {14, 23}]
```

Out[120]=

$$\left\{\frac{\mathbb{1}}{\sqrt{6}},\ -\frac{I^{-}\bullet S^{+}+I^{+}\bullet S^{-}+2\,(I_z\bullet S_z)}{2\sqrt{3}},\ \frac{S_z}{2},\ \sqrt{\frac{2}{3}}\,I_z,\ \frac{I^{-}\bullet S^{+}-I^{+}\bullet S^{-}}{2\sqrt{2}},\right.$$

$$-\frac{3\,(I^{-}\bullet S^{+}\bullet S_z)+3\,(I^{-}\bullet S_z\bullet S^{+})+3\,(I^{+}\bullet S^{-}\bullet S_z)+3\,(I^{+}\bullet S_z\bullet S^{-})-4\,(I_z\bullet S_x\bullet S_x)-4\,(I_z\bullet S_y\bullet S_y)+8\,(I_z\bullet S_z\bullet S_z)}{2\sqrt{30}},$$

$$-\frac{S_x\bullet S_x+S_y\bullet S_y-2\,(S_z\bullet S_z)}{2\sqrt{3}},\ -\frac{I^{-}\bullet S^{+}+I^{+}\bullet S^{-}-4\,(I_z\bullet S_z)}{2\sqrt{6}},\ \frac{I^{-}\bullet S^{+}\bullet S_z+I^{-}\bullet S_z\bullet S^{+}-I^{+}\bullet S^{-}\bullet S_z-I^{+}\bullet S_z\bullet S^{-}}{2\sqrt{2}},$$

$$\left.-\frac{I^{-}\bullet S^{+}\bullet S_z+I^{-}\bullet S_z\bullet S^{+}+I^{+}\bullet S^{-}\bullet S_z+I^{+}\bullet S_z\bullet S^{-}+2\,(I_z\bullet S_x\bullet S_x)+2\,(I_z\bullet S_y\bullet S_y)-4\,(I_z\bullet S_z\bullet S_z)}{2\sqrt{5}}\right\}$$

In[101]:=
```
MatrixForm[Simplify[Take[
   Normal[
    averageLiouvillianunderXY4element[
     -I CommutationSuperoperator["JIS" opI["I"].opI["S"]],
     freeevolutionsuperoperator (* free evolution *)
    ]], {14, 23}, {14, 23}]]]
```

Out[101]//MatrixForm=

$$\begin{pmatrix}
0 & 0 & 0 & 0 & 0 & 0 & 0 & 0 & 0 & 0\\
0 & 0 & 0 & 0 & 0 & 0 & 0 & 0 & 0 & 0\\
0 & 0 & 0 & 0 & \frac{i\,JIS}{\sqrt{2}} & 0 & 0 & 0 & 0 & 0\\
0 & 0 & 0 & 0 & -\frac{2\,i\,JIS}{\sqrt{3}} & 0 & 0 & 0 & 0 & 0\\
0 & 0 & \frac{i\,JIS}{\sqrt{2}} & -\frac{2\,i\,JIS}{\sqrt{3}} & 0 & -\frac{1}{2}\,i\sqrt{\frac{5}{3}}\,JIS & 0 & 0 & 0 & 0\\
0 & 0 & 0 & 0 & -\frac{1}{2}\,i\sqrt{\frac{5}{3}}\,JIS & 0 & 0 & 0 & 0 & 0\\
0 & 0 & 0 & 0 & 0 & 0 & 0 & 0 & i\sqrt{\frac{3}{2}}\,JIS & 0\\
0 & 0 & 0 & 0 & 0 & 0 & 0 & 0 & -\frac{1}{2}\,i\sqrt{3}\,JIS & 0\\
0 & 0 & 0 & 0 & 0 & 0 & i\sqrt{\frac{3}{2}}\,JIS & -\frac{1}{2}\,i\sqrt{3}\,JIS & 0 & 0\\
0 & 0 & 0 & 0 & 0 & 0 & 0 & 0 & 0 & 0
\end{pmatrix}$$

In[102]:=
```
MatrixForm[Simplify[Take[
   Normal[
    averageLiouvillianunderXY4element[
     -I CommutationSuperoperator["JIS" opI["I"].opI["S"]],
     rXY4Isup (* XY4(I) *)
    ]], {14, 23}, {14, 23}]]]
```

Out[102]//MatrixForm=

$$\begin{pmatrix} 0 & 0 & 0 & 0 & 0 & 0 & 0 & 0 & 0 & 0 \\ 0 & 0 & 0 & 0 & 0 & 0 & 0 & 0 & 0 & 0 \\ 0 & 0 & 0 & 0 & 0 & 0 & 0 & 0 & 0 & 0 \\ 0 & 0 & 0 & 0 & 0 & 0 & 0 & 0 & 0 & 0 \\ 0 & 0 & 0 & 0 & 0 & 0 & 0 & 0 & 0 & 0 \\ 0 & 0 & 0 & 0 & 0 & 0 & 0 & 0 & 0 & 0 \\ 0 & 0 & 0 & 0 & 0 & 0 & 0 & 0 & 0 & 0 \\ 0 & 0 & 0 & 0 & 0 & 0 & 0 & 0 & 0 & 0 \\ 0 & 0 & 0 & 0 & 0 & 0 & 0 & 0 & 0 & 0 \\ 0 & 0 & 0 & 0 & 0 & 0 & 0 & 0 & 0 & 0 \end{pmatrix}$$

In[103]:=
```
MatrixForm[Simplify[Take[
   Normal[
    averageLiouvillianunderXY4element[
     -I CommutationSuperoperator["JIS" opI["I"].opI["S"]],
     rXY4ISsup (* XY4(I+S) *)
    ]], {14, 23}, {14, 23}]]]
```

Out[103]//MatrixForm=

$$\begin{pmatrix} 0 & 0 & 0 & 0 & 0 & 0 & 0 & 0 & 0 & 0 \\ 0 & 0 & 0 & 0 & 0 & 0 & 0 & 0 & 0 & 0 \\ 0 & 0 & 0 & 0 & \frac{i\,\mathrm{JIS}}{\sqrt{2}} & 0 & 0 & 0 & 0 & 0 \\ 0 & 0 & 0 & 0 & -\frac{2\,i\,\mathrm{JIS}}{\sqrt{3}} & 0 & 0 & 0 & 0 & 0 \\ 0 & 0 & \frac{i\,\mathrm{JIS}}{\sqrt{2}} & -\frac{2\,i\,\mathrm{JIS}}{\sqrt{3}} & 0 & -\frac{1}{2}\,i\sqrt{\frac{5}{3}}\,\mathrm{JIS} & 0 & 0 & 0 & 0 \\ 0 & 0 & 0 & 0 & -\frac{1}{2}\,i\sqrt{\frac{5}{3}}\,\mathrm{JIS} & 0 & 0 & 0 & 0 & 0 \\ 0 & 0 & 0 & 0 & 0 & 0 & 0 & 0 & i\sqrt{\frac{3}{2}}\,\mathrm{JIS} & 0 \\ 0 & 0 & 0 & 0 & 0 & 0 & 0 & 0 & -\frac{1}{2}\,i\sqrt{3}\,\mathrm{JIS} & 0 \\ 0 & 0 & 0 & 0 & 0 & 0 & i\sqrt{\frac{3}{2}}\,\mathrm{JIS} & -\frac{1}{2}\,i\sqrt{3}\,\mathrm{JIS} & 0 & 0 \\ 0 & 0 & 0 & 0 & 0 & 0 & 0 & 0 & 0 & 0 \end{pmatrix}$$
